# Supplementary material for: Complex KDA: Understanding and Enhancing the Expressivity of Kimi Delta Attention
Source: arXiv:2609.24797 source file (2026-09-21)
Supplement: Supplementary file 2 [file appendix_efficient.tex]

\newpage
\definecolor{paperblue}{RGB}{200,220,255}
\tikzset{muted/.style={gray,opacity=0.5}}

\section*{\textbf{Supplementary Material}}
The supplementary material is structured as follows:
\begin{itemize}
    \item Section \ref{sec:bg} gives an overview on the background work on linear RNN variants and their expressivity.
    \item Section \ref{app:finite-group-expressivity} states the finite-group expressivity of one layer KDA, including $S_4$ and $A_5$.
    \item Section \ref{sec:setup} proves that only extending both the generalized Householder and diagonal gate parametric range leads to complex eigenvalues and therefore rotations that go beyond $180 \deg$ flips.
    \item Section \ref{app:wfamin} shows that only three layers of KDA in a transformer backbone (with sufficiently large feed forward networks are sufficient to model any Weighted Finite Automaton (given enough size).
    \item Section \ref{app:gauge} shows that through pulling out cumulative parities one can re-use existing KDA kernels, such that only a pre-transformation of queries and keys is needed
    \item Section \ref{app:silu} contains a short analysis on why not to use an activation function for keys.
    \item Section \ref{app:exp} states experimental details.
    \item Section \ref{appsec:exp_res} has additional experimental results.
    \item Section \ref{app:kernels} shows that fused kernels for signed KDA can stay within 97 \% of the speed of the existing KDA kernels
\end{itemize}

\textbf{LLM usage.} The change of variable described in~\Cref{app:gauge} to support signed gates without changes to the kernels was proposed by Claude Opus 5. The authors contextualized this idea among similar change of variables already used by other models. All proofs for the group word problem expressivity were done by GPT 5.6 Sol, then checked and quite heavily edited. Also, the proof adaption of three layers recognizing general WFAs of \citet{merrill_why_2026} in \ref{app:wfamin} was proposed by ChatGPT Sol, with edits made by Claude Opus 5. The theory in~\Cref{app:orthogonal-dplr} was developed during an exploration of the relationship between DPLR and signed KDA by the authors in collaboration with ChatGPT Sol.

\textbf{Notation.} We adopt the following notation throughout. Matrices are denoted by uppercase letters, such as $\mA$, $\mH$, and $\mM$, while vectors are represented by lowercase letters, such as $\vk$, $\vv$, and $\vx$. The sets of real and complex numbers are denoted by $\R$ and $\C$, respectively. The identity matrix is represented by $\mI$, and $\top$ denotes the transpose operator, so that, for example, $\vk^\top$ is the transpose of $\vk$. For a vector $\vv$, $\|\vv\|$ or $\|\vv\|_2$ denotes its Euclidean norm, whereas $\|\mA\|$ denotes the operator norm of a matrix $\mA$. The notation $|\cdot|$ represents the absolute value of a real scalar or the modulus of a complex number, and $\odot$ denotes the element-wise (Hadamard) product. Furthermore, $\spec(\mA)$ and $\rho(\mA)$ denote the spectrum, i.e., the set of eigenvalues, and the spectral radius of $\mA$, respectively. The symbols $\text{tr}(\mA)$ and $\det(\mA)$ denote the trace and determinant of $\mA$, respectively. Finally, $\ve_i \in \{0,1\}^n$ denotes the $i$-th vector of the canonical basis of $\R^n$.



\section{Background \& Related Work}\label{sec:bg}

Linear attention maintains a matrix-valued state $\mH_i\in\R^{n\times d_v}$ under the recurrence
$\mH_i=\mA_i\mH_{i-1}+\vk_i\vv_i^{\!\top}$, and the variants below differ mainly in the structure of
$\mA_i$. GLA~\citep{gla}, RWKV-6~\citep{peng2024eagle}, and HGRN-2~\citep{qin2024hgrn} all use diagonal state-transition matrices $\mA_i = \Diag(\valpha_i)$ whereas Mamba-2~\citep{dao2024transformers} and mLSTM~\citep{beck2024xlstm} use a simplified $\mA_i = \alpha_i\mI$ transition matrix. DeltaNet \citep{yang2024deltanet} takes $\mA_i=\mI-\beta_i\vk_i\vk_i^{\!\top}$ with
$\norm{\vk_i}_2=1$, a generalised Householder matrix that replaces the value stored at $\vk_i$ rather
than adding to it. Gated DeltaNet \citep{yang2025gdn} multiplies this by a scalar decay
$\alpha_i\in(0,1)$, and KDA \citep{kimi2025} replaces that scalar by a channel-wise gate. All three are instances of the diagonal-plus-low-rank (DPLR) family
$\mA_i=\mD_i-\va_i\vb_i^{\!\top}$, which is what admits the chunkwise WY representation~\citep{wy_representation} these models rely
on for training throughput.

Recent variants each modify one component of the state-transition matrix.
Solar Open~2 \citep{upstage2026} widens the learning rate to $\beta\in(0,2)$, following the
negative-eigenvalue argument of \citet{grazzi2025}; \citet{yang2025path} adopt the same range in a
position-encoding role. Three variants refine the granularity of the write. FG$^2$-GDN
\citep{fg2gdn2026} makes $\beta$ channel-wise, absorbing it symmetrically into the key as
$\tilde\vk_i=\sqrt{\vb_i}\odot\vk_i$ so that the rank-one factor stays a symmetric projector and the
KDA kernel is preserved; FG$^2$-GDN+ additionally decouples the scaling of keys and values; and
Gated DeltaNet-2 \citep{hatamizadeh2026gdn2} separates a channel-wise erase gate on the key axis from
a channel-wise write gate on the value axis. Two variants change the field or the order of the
recurrence: SFDA \citep{zhang2026sfda} replaces the real diagonal with a complex Fourier gate
$\Diag(\valpha_i\odot e^{i\vtheta_i})$, and MDN \citep{huang2026} adds a momentum term
$-\tilde\gamma_i\mH_{i-2}$, doubling the state. RWKV-7 \citep{peng2025rwkv7} sits slightly outside
this lineage: its transition is also DPLR, but the diagonal is carried by the rank-one term rather
than applied after it.

The modification studied here widens the
\emph{range} of the decay gate rather than its granularity, the one axis none of these variants has
altered. 


\begin{figure}
    \centering
    \includegraphics[width=1.0\linewidth]{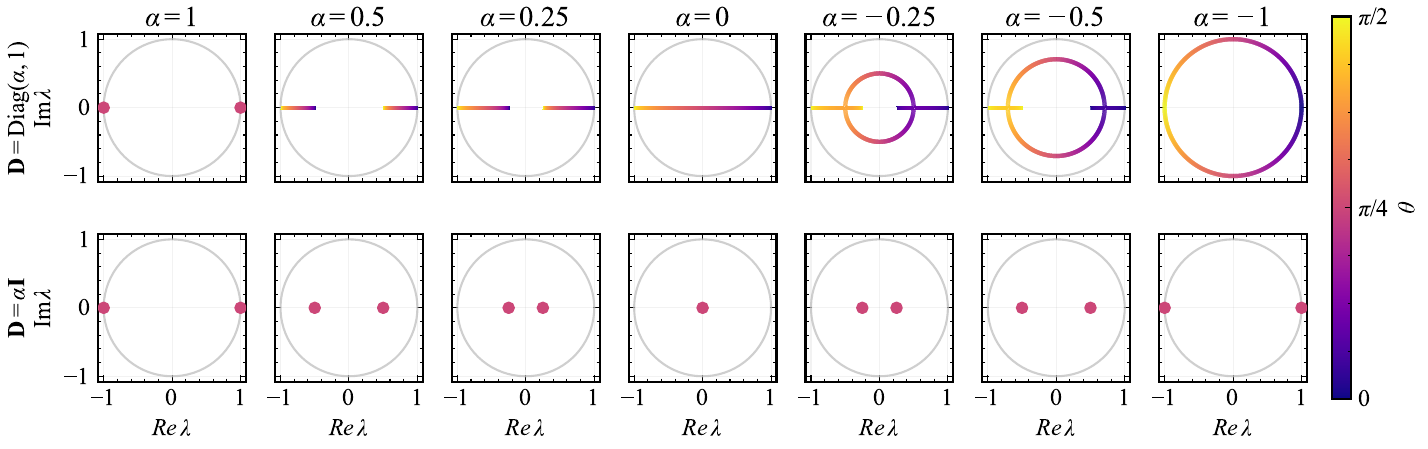}
    \vspace{-8mm}
\caption{Spectral view of the two-dimensional construction. For
$\mA=(\mI-2\vk\vk^\top)\mD$ with
$\vk=(\cos\theta,\sin\theta)^\top$ and
$\theta\in[0,\pi/2]$, we vary $\alpha$ from $1$ to $-1$.
Top: for the channel-wise gate $\mD=\Diag(\alpha,1)$,
a complex-conjugate pair appears when $\alpha<0$ and reaches the
unit circle at $\alpha=-1$, recovering the rotation family. Bottom: for the scalar gate
$\mD=\alpha\mI$, the spectrum remains real throughout.}
\label{fig:alpha_sweep_2d}
\end{figure}

\section{Finite-group expressivity of one layer KDA}
\label{app:finite-group-expressivity}


Consider a state-tracking problem in which each input is an element of a
finite group $G$.  After reading $g_1,\ldots,g_t$, the state to be tracked is
their product.  A standard exact linear construction chooses a faithful
orthogonal representation $\rho:G\to O(d)$.  Here \emph{homomorphism} means
that $\rho$ preserves multiplication,
\[
  \rho(gh)=\rho(g)\rho(h)\qquad(g,h\in G),
\]
and \emph{faithful} means that distinct group elements have distinct matrix
representations,
\[
  \rho(g)=\rho(h)\Longrightarrow g=h.
\]
The construction
then updates
\[
  \mX_t=\rho(g_t)\mX_{t-1},\qquad \mX_0=\mI.
\]
We ask when all of these update
matrices can be chosen from one restricted family.

For $\vu\in\R^d$ with $\|\vu\|=1$, the Householder matrix
\[
  \mH_{\vu}:=\mI-2\vu\vu^\top
\]
is the reflection in the hyperplane $\vu^\perp$.  A \emph{sign diagonal} is
\[
  \mD=\Diag(\varepsilon_1,\ldots,\varepsilon_d),
  \qquad \varepsilon_i\in\{-1,+1\}.
\]
We call a product $\mH_{\vu}\mD$ a \emph{signed-Householder matrix}.  Such
matrices do not themselves form a group.  Our question is only whether the
matrices representing all elements of a given group can have this form.

\theoremstyle{definition}
\newtheorem{definition}{Definition}[section]  %

\begin{definition}[signed-Householder realization]\leavevmode\par
A finite group $G$ admits a \emph{signed-Householder realization} if there
are a dimension $d$ and a faithful homomorphism $\rho:G\to O(d)$ such that,
for every $g\in G$, there are a sign diagonal $\mD_g$ and a unit vector $\vu_g$
satisfying
\[
  \rho(g)=\mH_{\vu_g}\mD_g.
\]
\end{definition}

This is exactly the KDA order.  The identity is allowed: with
$\mD_1:=\Diag(-1,1,\ldots,1)=\mH_{\ve_1}$, we have
$\mI=\mH_{\ve_1}\mD_1$.  Section~\ref{app:icosahedron} contrasts this faithful
matrix question with exact state tracking under a many-to-one decoder.

\subsection{Signed-Householder 3D rotations' axis lies in a coordinate plane}\label{app:axis-test}

A rotation in $\R^3$ fixes its axis and rotates the perpendicular plane.
The following proposition characterizes exactly when such a rotation is a
signed-Householder matrix.  Its proof uses only the elementary fact that
the product of reflections in two planes is a rotation about their line of
intersection.


\begin{proposition}[axis test]\label{prop:axis-test}
Let $\mR\in SO(3)$ be a rotation about the axis $\R\va$.
\begin{enumerate}
  \item The identity and every half-turn have the form $\mH_{\vu}\mD$.
  \item If its angle is different from $0$ and $\pi$, then
  $\mR=\mH_{\vu}\mD$ for some sign diagonal $\mD$ if and only if its axis
  is contained in a coordinate plane.  Explicitly, this means that
  $\va\perp\ve_i$ for some coordinate axis $\R\ve_i$, or equivalently that
  $\va$ has at least one zero coordinate.
\end{enumerate}
\end{proposition}

\begin{proof}
For part 1, the matrix $2\va\va^\top-\mI$ fixes $\va$ and sends every
$\vx\perp\va$ to $-\vx$, so it is the half-turn about $\R\va$.  Moreover,
\[
  2\va\va^\top-\mI=(\mI-2\va\va^\top)(-\mI)=\mH_{\va}(-\mI),
\]
which has the required form.  The identity does as well: with
$\mD_1:=\Diag(-1,1,1)=\mH_{\ve_1}$, we have
$\mI=\mH_{\ve_1}\mD_1$.

For part 2, suppose $\mR=\mH_{\vu}\mD$.  Since
$\det\mH_{\vu}=-1$ and $\det\mR=1$, the diagonal $\mD$ has either one or
three negative entries.  In the latter case $\mD=-\mI$ and
$\mR=2\vu\vu^\top-\mI$, the half-turn from part 1, contradicting the
assumption on the angle.  Hence $\mD$ has exactly one negative entry.
If that entry is in position $i$, then
$\mD=\mI-2\ve_i\ve_i^\top$, which is precisely the reflection across the
coordinate plane $\ve_i^\perp$.

Both factors are now reflections in planes: $\mD$ reflects in
$\ve_i^\perp$ and $\mH_{\vu}$ reflects in $\vu^\perp$.  Their product
rotates about the line $\ve_i^\perp\cap\vu^\perp$.  This is the axis
$\R\va$, so $\va\perp\ve_i$; in other words, $\va$ lies in the coordinate
plane $\ve_i^\perp$.

Conversely, every rotation in $SO(3)$ is a product of reflections in two
planes through its axis, separated by half the rotation angle.  If
$\va\perp\ve_i$, we may choose one plane to be the coordinate plane
$\ve_i^\perp$.  Its reflection is
$\mD_i=\mI-2\ve_i\ve_i^\top$; the other reflection is therefore
$\mH_{\vu}:=\mR\mD_i$, and $\mR=\mH_{\vu}\mD_i$.
\end{proof}

\subsection{Cyclic and dihedral groups}\label{app:planar-groups}

\begin{proposition}[planar groups]\label{prop:planar-groups}
Every cyclic group $\mathbb{Z}_n$ and every dihedral group $D_n$ has a
signed-Householder realization in two dimensions.
\end{proposition}

\begin{proof}
In the plane, take $\mD_0=\Diag(1,-1)$, reflection in the horizontal axis.
If $\mS_\alpha$ denotes reflection in the line making angle $\alpha$ with
the horizontal axis, then $\mS_\alpha\mD_0$ is a rotation through $2\alpha$.
Choosing $\alpha=\pi k/n$ realizes every rotation through $2\pi k/n$, so
every element in the standard representation of $\mathbb{Z}_n$ has the required
form.

The dihedral group adds reflections of the regular $n$-gon.  Each is already
a Householder matrix, so choose $\mD=\mI$.  Thus the same is true for the
standard planar representation of $D_n$.
\end{proof}

\subsection{Realizing \texorpdfstring{$S_4$}{S4} via the cube rotational symmetries}\label{app:cube}

The group $S_4$ has a familiar geometric realization: it is isomorphic to
the group of rotational symmetries of a cube.  We now show that rotating the
cube to a suitable orientation makes all of these rotations admissible at
once.

Figure~\ref{fig:cube-axis-types} shows the face and body-diagonal axes;
edge axes give only half-turns.

\begin{figure}[!ht]
\centering
\begin{tikzpicture}[>=Latex,font=\small,scale=.86,transform shape]
\fill[paperblue,rounded corners=5pt] (-7.2,-2.0) rectangle (7.2,2.15);

\begin{scope}[shift={(-4.6,.12)},
  x={(.640679cm,.207183cm)},
  y={(-.427119cm,.310775cm)},
  z={(0cm,.673345cm)}]
  \coordinate (ca) at (-1,-1,-1); \coordinate (cb) at (1,-1,-1);
  \coordinate (cc) at (1,1,-1);   \coordinate (cd) at (-1,1,-1);
  \coordinate (ce) at (-1,-1,1);  \coordinate (cf) at (1,-1,1);
  \coordinate (cg) at (1,1,1);    \coordinate (ch) at (-1,1,1);
  \foreach \a/\b in {cb/cc,cc/cd,cc/cg}
    \draw[muted,densely dashed,line width=.55pt] (\a)--(\b);
  \foreach \a/\b in {ca/cb,cd/ca,ce/cf,cf/cg,cg/ch,ch/ce,
                       ca/ce,cb/cf,cd/ch}
    \draw[ink,line width=.9pt] (\a)--(\b);
\end{scope}
\node[text=ink,font=\bfseries\scriptsize] at (-4.6,-1.52) {Cube};

\begin{scope}[shift={(0,.1)}]
  \draw[ink,line width=.9pt] (0,-1.088944)--(1.088944,0)--
    (0,1.088944)--(-1.088944,0)--cycle;
  \fill[bad] (0,0) circle (2.4pt);
  \draw[bad,very thick,->] (0:1.54)
    arc[start angle=0,end angle=90,radius=1.54];
  \node[text=bad,font=\bfseries\footnotesize]
    at (45:2.09) {$90^\circ$};
\end{scope}
\node[text=ink,font=\bfseries\scriptsize] at (0,-1.52) {Face axis: order $4$};

\begin{scope}[shift={(4.6,.1)},x={(1.257405cm,0cm)},y={(0cm,1.257405cm)}]
  \coordinate (cv2) at (0,-1);          \coordinate (cv3) at (-.866025,.5);
  \coordinate (cv4) at (-.866025,-.5);  \coordinate (cv5) at (.866025,.5);
  \coordinate (cv6) at (.866025,-.5);   \coordinate (cv7) at (0,1);
  \draw[ink,line width=.9pt] (cv2)--(cv6)--(cv5)--(cv7)--(cv3)--(cv4)--cycle;
  \draw[muted,densely dashed,line width=.55pt]
    (0,0)--(cv2) (0,0)--(cv3) (0,0)--(cv5);
  \draw[ink,line width=.85pt] (0,0)--(cv4) (0,0)--(cv6) (0,0)--(cv7);
  \fill[bad] (0,0) circle (2.4pt);
  \draw[bad,very thick,->] (-30:1.30)
    arc[start angle=-30,end angle=90,radius=1.30];
  \node[text=bad,font=\bfseries\footnotesize]
    at (30:1.80) {$120^\circ$};
\end{scope}
\node[text=ink,font=\bfseries\scriptsize] at (4.6,-1.52) {Vertex axis: order $3$};
\end{tikzpicture}
\caption{Smallest symmetry-preserving rotations (excluding half-turns) for the Cube, grouped by axis. The red point marks the axis viewed end-on; visible edges are solid and hidden edges are dashed.}
\label{fig:cube-axis-types}
\end{figure}

\begin{proposition}[cube realization]\label{prop:cube}
The group $S_4$, realized as the rotational symmetry group of a cube, has a
signed-Householder realization in three dimensions.
\end{proposition}

\begin{proof}
The orientation-preserving symmetry group of a cube is isomorphic to
$S_4$: it permutes the four unoriented body diagonals faithfully.  Its
non-half-turn rotation axes are
\begin{itemize}
  \item the three face axes, supporting quarter-turns; and
  \item the four body diagonals, supporting rotations through
  $\pm 2\pi/3$.
\end{itemize}
All remaining non-identity rotations are half-turns and are automatically
admissible by Proposition~\ref{prop:axis-test}.

Place the cube first in its standard orientation.  The three face axes and
four body-diagonal axes are represented, respectively, by
\[
 \mathcal F=\{(1,0,0),(0,1,0),(0,0,1)\},\qquad
 \mathcal B=\{(1,1,1),(1,1,-1),(1,-1,1),(-1,1,1)\}.
\]
Every vector in $\mathcal B$ has three nonzero coordinates, so this
orientation does not pass the axis test of
Proposition~\ref{prop:axis-test}.  Now rotate the cube by $45^\circ$
about the third coordinate axis, using
\[
 \mR=\begin{pmatrix}
  1/\sqrt2& 1/\sqrt2&0\\
 -1/\sqrt2& 1/\sqrt2&0\\
  0&0&1
 \end{pmatrix}\in SO(3).
\]
Applying $\mR$ to each of the seven axes gives
\[
 \begin{aligned}
 \mR\mathcal F&=
 \left\{\frac{(1,-1,0)}{\sqrt2},\frac{(1,1,0)}{\sqrt2},(0,0,1)\right\},\\
 \mR\mathcal B&=\{(\sqrt2,0,1),(\sqrt2,0,-1),
 (0,-\sqrt2,1),(0,\sqrt2,1)\}.
 \end{aligned}
\]
Thus the rotation does not spoil the three face axes: they still have a zero
coordinate, as do all four transformed body diagonals.  Proposition~
\ref{prop:axis-test} therefore shows that every cube rotation is a
signed-Householder matrix.
\end{proof}


\subsection{\texorpdfstring{How to track $A_5$}{A5}}\label{app:icosahedron}

The orientation-preserving symmetry group of the icosahedron is isomorphic to $A_5$.
This section has one negative and one positive result.  The negative result
rules out every finite orthogonal hidden group in three dimensions, even if
the decoder is an arbitrary function.  The positive
result then constructs an exact four-dimensional tracker by allowing several
hidden matrices to decode to the same $A_5$ element.

An icosahedron has $12$ vertices, $20$ faces, and $30$ edges.  Pairing each
feature with its opposite gives the rotation axes below.  An axis has
\emph{order $k$} if the rotations about it form a cyclic group of $k$
elements; equivalently, its smallest positive rotation has angle $2\pi/k$
and returns to the identity after $k$ applications.  Thus there are
\[
  6\text{ axes of order }5,\qquad
  10\text{ axes of order }3,\qquad
  15\text{ axes of order }2.
\]
The order-$2$ axes do not matter, since half-turns are always in the required form (Proposition~\ref{prop:axis-test}).  The difficulty comes from the other sixteen axes.
Figure~\ref{fig:ico-axis-types} illustrates these two relevant axis types.

\begin{figure}[!ht]
\centering
\begin{tikzpicture}[>=Latex,font=\small,scale=.86,transform shape]
\fill[paperblue,rounded corners=5pt] (-6.9,-1.82) rectangle (6.9,2.02);

\begin{scope}[shift={(-4.6,.18)},
  x={(.437287cm,.164688cm)},
  y={(-.349829cm,.205860cm)},
  z={(0cm,.494064cm)}]
  \coordinate (ia1) at (0,1,1.618);   \coordinate (ia2) at (0,-1,1.618);
  \coordinate (ia3) at (0,1,-1.618);  \coordinate (ia4) at (0,-1,-1.618);
  \coordinate (ia5) at (1,1.618,0);   \coordinate (ia6) at (-1,1.618,0);
  \coordinate (ia7) at (1,-1.618,0);  \coordinate (ia8) at (-1,-1.618,0);
  \coordinate (ia9) at (1.618,0,1);   \coordinate (ia10) at (-1.618,0,1);
  \coordinate (ia11) at (1.618,0,-1); \coordinate (ia12) at (-1.618,0,-1);
  \foreach \a/\b in {ia1/ia5,ia3/ia4,ia3/ia5,
    ia3/ia6,ia3/ia11,ia3/ia12,ia4/ia11,ia5/ia6,ia5/ia9,
    ia5/ia11,ia7/ia11,ia9/ia11}
    \draw[muted,densely dashed,line width=.42pt] (\a)--(\b);
  \foreach \a/\b in {ia1/ia2,ia1/ia6,ia1/ia9,ia1/ia10,
    ia2/ia7,ia2/ia8,ia2/ia9,ia2/ia10,ia4/ia7,ia4/ia8,
    ia4/ia12,ia6/ia10,ia7/ia8,ia6/ia12,ia7/ia9,ia8/ia10,
    ia8/ia12,ia10/ia12}
    \draw[ink,line width=.68pt] (\a)--(\b);
\end{scope}
\node[text=ink,font=\bfseries\scriptsize] at (-4.6,-1.4) {Icosahedron};

\begin{scope}[shift={(0,.18)},x={(.56cm,0cm)},y={(0cm,.56cm)}]
  \coordinate (iaf1) at (-1,-.577350);       \coordinate (iaf2) at (0,-1.868345);
  \coordinate (iaf3) at (0,1.868345);        \coordinate (iaf4) at (1,.577350);
  \coordinate (iaf5) at (0,1.154701);        \coordinate (iaf6) at (-1.618034,.934172);
  \coordinate (iaf7) at (1.618034,-.934172); \coordinate (iaf8) at (0,-1.154701);
  \coordinate (iaf9) at (1,-.577350);        \coordinate (iaf10) at (-1.618034,-.934172);
  \coordinate (iaf11) at (1.618034,.934172); \coordinate (iaf12) at (-1,.577350);
  \foreach \a/\b in {iaf2/iaf8,iaf3/iaf4,iaf3/iaf12,iaf4/iaf7,
    iaf4/iaf8,iaf4/iaf11,iaf4/iaf12,iaf6/iaf12,iaf7/iaf8,
    iaf8/iaf10,iaf8/iaf12,iaf10/iaf12}
    \draw[muted,densely dashed,line width=.4pt] (\a)--(\b);
  \foreach \a/\b in {iaf1/iaf2,iaf1/iaf5,iaf1/iaf6,iaf1/iaf9,
    iaf1/iaf10,iaf2/iaf7,iaf2/iaf9,iaf2/iaf10,iaf3/iaf5,
    iaf3/iaf6,iaf3/iaf11,iaf5/iaf6,iaf5/iaf9,iaf5/iaf11,
    iaf6/iaf10,iaf7/iaf9,iaf7/iaf11,iaf9/iaf11}
    \draw[ink,line width=.62pt] (\a)--(\b);
  \draw[ink,line width=1pt] (iaf1)--(iaf5)--(iaf9)--cycle;
  \fill[bad] (0,0) circle (2.4pt);
  \draw[bad,very thick,->] (-30:2.42)
    arc[start angle=-30,end angle=90,radius=2.42];
  \node[text=bad,font=\bfseries\footnotesize]
    at (30:3.44) {$120^\circ$};
\end{scope}
\node[text=ink,font=\bfseries\scriptsize] at (0,-1.4) {Face axis: order $3$};

\begin{scope}[shift={(4.6,.18)},x={(.56cm,0cm)},y={(0cm,.56cm)}]
  \coordinate (iav1) at (0,0);             \coordinate (iav2) at (0,-1.701302);
  \coordinate (iav3) at (0,1.701302);      \coordinate (iav4) at (0,0);
  \coordinate (iav5) at (1,1.376382);      \coordinate (iav6) at (-1,1.376382);
  \coordinate (iav7) at (1,-1.376382);     \coordinate (iav8) at (-1,-1.376382);
  \coordinate (iav9) at (1.618034,-.525731);\coordinate (iav10) at (-1.618034,-.525731);
  \coordinate (iav11) at (1.618034,.525731);\coordinate (iav12) at (-1.618034,.525731);
  \foreach \a/\b in {iav3/iav4,iav3/iav11,iav3/iav12,iav4/iav7,
    iav4/iav8,iav4/iav11,iav4/iav12,iav7/iav8,iav7/iav11,
    iav8/iav12}
    \draw[muted,densely dashed,line width=.4pt] (\a)--(\b);
  \foreach \a/\b in {iav1/iav2,iav1/iav5,iav1/iav6,iav1/iav9,
    iav1/iav10,iav2/iav7,iav2/iav8,iav2/iav9,iav2/iav10,
    iav3/iav5,iav3/iav6,iav5/iav6,iav5/iav9,iav5/iav11,
    iav6/iav10,iav6/iav12,iav7/iav9,iav8/iav10,iav9/iav11,
    iav10/iav12}
    \draw[ink,line width=.62pt] (\a)--(\b);
  \fill[bad] (0,0) circle (2.4pt);
  \draw[bad,very thick,->] (-18:2.44)
    arc[start angle=-18,end angle=54,radius=2.44];
  \node[text=bad,font=\bfseries\footnotesize]
    at (18:3.47) {$72^\circ$};
\end{scope}
\node[text=ink,font=\bfseries\scriptsize] at (4.6,-1.4) {Vertex axis: order $5$};
\end{tikzpicture}
\caption{Smallest symmetry-preserving rotations (excluding half-turns) for the Icosahedron, grouped by axis. The red point
marks the axis viewed end-on; visible edges are solid and hidden edges are
dashed.}
\label{fig:ico-axis-types}
\end{figure}


By the axis test (Proposition~\ref{prop:axis-test}), representing all
odd-order rotations would require three coordinate planes to cover all
sixteen axes.  We prove the stronger,
orientation-independent fact that \emph{any} plane covers at most four.

\subsubsection{$A_5$ can't be tracked in 3 dimensions}

\begin{lemma}[icosahedral plane bound]\label{lem:ico-plane}
Among the six order-$5$ axes and ten order-$3$ axes of an icosahedron, no
plane through the centre contains more than four axes.
\end{lemma}

\begin{proof}
Let $\varphi=(1+\sqrt5)/2$ be the golden ratio.  In the usual coordinates, representative vectors for
the six unoriented vertex axes (the order-$5$ axes) are
\[
\mathcal V=
\left\{
(0,1,\pm\varphi),\ (1,\pm\varphi,0),\ (\varphi,0,\pm1)
\right\}.
\]
The face centres form the vertices of the dual dodecahedron. Representatives
of their ten unoriented axes (the order-$3$ axes) are
\[
\begin{split}
\mathcal T={}&\{(1,1,1),(1,1,-1),(1,-1,1),(-1,1,1)\}\\
&\cup\{(0,\varphi-1,\pm\varphi),
       (\varphi-1,\pm\varphi,0),
       (\varphi,0,\pm(\varphi-1))\}.
\end{split}
\]
It suffices to check that no three axes in either family are coplanar.
Indeed, substituting the displayed vectors and using
$\varphi^2=\varphi+1$ gives the following possible absolute determinants
of three distinct representatives:
\[
\begin{array}{c@{\qquad}l}
\toprule
\text{family}&|\det(\vv_1,\vv_2,\vv_3)|\\
\midrule
\mathcal V&1+\sqrt5,\ 3+\sqrt5\\
\mathcal T&\sqrt5-1,\ 2,\ 1+\sqrt5,\ 2\sqrt5,\ 4\\
\bottomrule
\end{array}
\]
All these determinants are nonzero.  Thus a plane contains at most two vertex
axes and at most two face axes, hence at most four axes in total.  Note, the bound
is tight: the plane $x=0$ contains
\[
 (0,1,\varphi),\ (0,1,-\varphi),\
 (0,\varphi-1,\varphi),\ (0,\varphi-1,-\varphi).
\]
\end{proof}

\begin{theorem}[$A_5$ Can't be tracked in three dimensions]\label{thm:a5-three}
There is no faithful homomorphism $\rho:A_5\to O(3)$ for which every
$\rho(g)$ is a signed-Householder matrix.

More generally, let $\Gamma \subset O(3)$ be a finite group generated by token
matrices $\{\mA_g:g\in A_5\}$, each of which is signed-Householder.  There is
no function $p:\Gamma\to A_5$ satisfying
\begin{equation}\label{eq:3d-arbitrary-decoder}
  p(\mI)=e,\qquad p(\mA_g\mQ)=g\,p(\mQ)
  \quad(g\in A_5,\ \mQ\in\Gamma).
\end{equation}
Thus no finite orthogonal three-dimensional hidden-group tracker works even
with an arbitrary decoder.
\end{theorem}

\begin{proof}
We first prove the faithful statement.
Let $\rho:A_5\to O(3)$ be faithful.  The map \(g\mapsto \det\rho(g)\) is a homomorphism from \(A_5\) to
\(\{\pm1\}\). Since \(A_5\) is simple, its kernel is either trivial or all of
\(A_5\); the former is impossible, as it would make \(A_5\) isomorphic to a
subgroup of \(\{\pm1\}\). Hence the kernel is all of \(A_5\), so
\(\det\rho(g)=1\) for every \(g\in A_5\).  Thus $\rho(A_5)\subset SO(3)$.  Up to an orthogonal change of
coordinates, every subgroup of $SO(3)$ isomorphic to $A_5$ is the rotation
group of an icosahedron.  It therefore suffices to consider an arbitrary
orientation of that solid.

Three coordinate planes can cover at most $3\cdot4=12$ of the sixteen
odd-order axes, by Lemma~\ref{lem:ico-plane}.  Thus at least four axes remain
outside, regardless of how the icosahedron is oriented.  The axis test
(Proposition~\ref{prop:axis-test}) says that the rotations about those axes
cannot have the required signed-Householder form. This proves the first statement.

Now suppose that a finite group $\Gamma$ and a completely arbitrary function
$p$ satisfy \eqref{eq:3d-arbitrary-decoder}.  Since $\Gamma$ is finite and
generated by the $\mA_g$, iterating \eqref{eq:3d-arbitrary-decoder} extends it
from the generators to all $\mQ_1\in\Gamma$, so
$p(\mQ_1\mQ_2)=p(\mQ_1)p(\mQ_2)$.  Thus $p$ is a homomorphism, and it is
surjective because $p(\mA_g)=g$.

Since $\Gamma\subset O(3)$, $\Gamma^+=\Gamma\cap SO(3)$ is the kernel of
$\det|_\Gamma:\Gamma\to\{\pm1\}$, hence is normal of index at most two.  Thus
$p(\Gamma^+)$ is normal in $A_5$ (the image of a normal subgroup under a
surjective homomorphism is normal).  This image cannot be trivial: otherwise
$p$ would be constant on cosets of $\Gamma^+$ and hence factor through
$\Gamma/\Gamma^+$, a group of order at most two.  Simplicity of $A_5$ therefore
forces $p(\Gamma^+)=A_5$.  The classification of finite subgroups of $SO(3)$ now
shows that $\Gamma^+\cong A_5$: the other possibilities are cyclic,
dihedral, $A_4$, and $S_4$, all solvable, whereas a quotient of a solvable
group is solvable and $A_5$ is not.  Thus
$|\Gamma^+|=|A_5|=60$, and the surjective restriction
$p|_{\Gamma^+}:\Gamma^+\to A_5$ is an isomorphism.  Write
\[
  \rho=(p|_{\Gamma^+})^{-1}:A_5\longrightarrow\Gamma^+.
\]

It remains to compare each token with this faithful icosahedral copy.  Put
$\mathbf Z_g=\mA_g\rho(g)^{-1}$.  Since $p(\mA_g)=p(\rho(g))=g$, we have
$p(\mathbf Z_g)=gg^{-1}=e$, hence $\mathbf Z_g\in\ker p$.  Moreover,
$p|_{\Gamma^+}$ is injective, so
$\ker p\cap\Gamma^+=\{\mI\}$.  Hence two elements of $\ker p$ with the same
determinant must be equal (their quotient lies in this intersection), and
$|\ker p|\leq2$.  If the kernel contains an orientation-reversing element
$\mathbf Z$, it is therefore unique.  As a kernel, $\ker p$ is normal: this
means that $\mR\mathbf Z\mR^{-1}\in\ker p$ for every $\mR\in\Gamma$.
Conjugation preserves the determinant, so for $\mR\in\Gamma^+$ this is again
the unique orientation-reversing kernel element, and hence
$\mR\mathbf Z\mR^{-1}=\mathbf Z$.  Thus $\mathbf Z$ lies in the centralizer of
$\Gamma^+$ in $O(3)$, namely the set of orthogonal matrices that commute with
every element of $\Gamma^+$.

This centralizer is $\{\pm\mI\}$.  Indeed, a commuting orthogonal map must
preserve the axis of each order-$5$ rotation (its one-dimensional fixed
space).  Choose three such axes that span $\R^3$ and are pairwise
nonorthogonal, with unit vectors $\vu_1,\vu_2,\vu_3$.  On each invariant line,
$\mathbf Z\vu_i=\varepsilon_i\vu_i$ for some $\varepsilon_i\in\{\pm1\}$.
Because $\mathbf Z$ preserves inner products and
$\langle\vu_i,\vu_j\rangle\ne0$, we have
$\varepsilon_i\varepsilon_j=1$ for every $i\ne j$.  All three signs are
therefore equal, so $\mathbf Z=\pm\mI$.  Since $\mathbf Z$ reverses
orientation, it must be $\mathbf Z=-\mI$.
Consequently, in all cases,
\[
  \mA_g\in\{\rho(g),-\rho(g)\}\qquad(g\in A_5).
\]
Multiplication by $-\mI$ does not change whether a matrix is
signed-Householder: if $\mA=\mH_{\vu}\mD$, then
$-\mA=\mH_{\vu}(-\mD)$.  Thus every $\rho(g)$ would be
signed-Householder, contradicting the faithful obstruction proved above.
\end{proof}

\subsubsection{A four-dimensional construction that tracks $A_5$}\label{app:A5const}

The preceding theorem shows that a non-injective decoder cannot rescue a
finite orthogonal hidden group in three dimensions.  Four dimensions do
admit such a finite extension.  We state the result using the actual KDA
readout.  Let the matrix state update as \(\mS\mapsto\mA_g\mS\), fix a query
\(\mathbf q\), and let
\(\mathcal O=\{\mS^\top\mathbf q:\mS\text{ is reachable}\}\) be the set of
query outputs.  The recurrence tracks the group exactly if there is a
surjection
\begin{equation}\label{eq:tracking-quotient}
  \pi:\mathcal O\longrightarrow A_5,\qquad
  \pi(\mathbf q)=e,\qquad
  \pi((\mA_g\mS)^\top\mathbf q)
  =g\,\pi(\mS^\top\mathbf q).
\end{equation}
This is the automaton-homomorphism definition used for state tracking: the
decoder sees only the standard KDA output and may map several outputs to the
same group element.

\begin{theorem}[four-dimensional \(A_5\) tracker]\label{thm:a5-four}
There are sixty matrices \(\{\mA_g:g\in A_5\}\subset SO(4)\) of the form
\[
  \mA_g=(\mI-2\va_g\va_g^\top)\Diag(-1,1,1,1),
  \qquad \|\va_g\|=1,
\]
such that one stable extended-KDA layer tracks the full \(A_5\) word problem
exactly from the standard query output \(\mS_t^\top\mathbf q\), using one
fixed query.  The reachable set is finite, so the construction has fixed
precision, and the output decoder is genuinely many-to-one.
\end{theorem}

\begin{proof}
We build the tracker in six steps.

\paragraph{Step 1: lift the icosahedral rotations to 120 unit quaternions.}
Identify \(\R^4\) with the quaternions
\[
  \mathbb H=\{w+x\mathrm i+y\mathrm j+z\mathrm k\},
  \qquad |q|^2=q\bar q=w^2+x^2+y^2+z^2.
\]
The unit quaternions form \(S^3\).  They act on the imaginary quaternions
\(\operatorname{Im}\mathbb H\cong\R^3\) by
\begin{equation}\label{eq:quaternion-cover}
  \kappa(a)(v)=ava^{-1}.
\end{equation}
The map \(\kappa:S^3\to SO(3)\) is a surjective homomorphism with kernel
\(\{\pm1\}\).  Therefore the full lift of the icosahedral rotation group,
\[
  \widetilde A_5:=\kappa^{-1}(A_5),
\]
is a group of \(120\) unit quaternions, called the binary icosahedral group,
and
\begin{equation}\label{eq:binary-quotient}
  \widetilde A_5/\{\pm1\}\cong A_5.
\end{equation}

\paragraph{Step 2: choose one lift for each of the 60 tokens.}
If \(g\neq e\) rotates through angle \(\theta_g\in(0,\pi]\) about the
oriented unit axis
\(\mathbf n_g=(n_{g,1},n_{g,2},n_{g,3})\), choose
\begin{equation}\label{eq:explicit-lift}
  \va_g=
  \cos\frac{\theta_g}{2}
  +\sin\frac{\theta_g}{2}
   (n_{g,1}\mathrm i+n_{g,2}\mathrm j+n_{g,3}\mathrm k),
\end{equation}
and set \(\va_e=1\).  Then \(\kappa(\va_g)=g\).  The only other choice is
\(-\va_g\), which will produce the same Householder matrix.

\paragraph{Step 3: turn every lift into one KDA transition.}
Let \(\ve=1=(1,0,0,0)\).  Since
\(\mH_{\ve}=\Diag(-1,1,1,1)\), define
\begin{equation}\label{eq:a5-transition}
  \mA_g:=\mH_{\va_g}\mH_{\ve}
  =(\mI-2\va_g\va_g^\top)\Diag(-1,1,1,1).
\end{equation}
Thus every token uses the same diagonal gate and only the Householder normal
changes.  Each \(\mA_g\) is the product of two reflections, so
\(\mA_g\in SO(4)\).

There is also a useful formula for its action.  For unit \(\va\),
\[
  \mH_{\va}(q)=-\va\bar q\va,
  \qquad \mH_{\ve}(q)=-\bar q.
\]
Consequently
\begin{equation}\label{eq:binary-update}
  \mA_g(q)=\va_gq\va_g.
\end{equation}
The right-hand side means two Hamilton products,
\[
  \va_gq\va_g
  =(\va_g\mathbin{\ast_{\mathbb H}}q)
     \mathbin{\ast_{\mathbb H}}\va_g,
\]
not coordinatewise multiplication in \(\R^4\).

\paragraph{Step 4: understand arbitrary products.}
For \(L,R\in\widetilde A_5\), write
\[
  \Phi_{L,R}(q):=LqR.
\]
These are orthogonal four-dimensional rotations, and direct substitution
gives
\begin{align}
  \Phi_{L_1,R_1}\Phi_{L_2,R_2}
    &=\Phi_{L_1L_2,R_2R_1},\label{eq:pair-composition}\\
  \Phi_{L,R}^{-1}&=\Phi_{L^{-1},R^{-1}}.
\end{align}
Hence the maps are closed under products and inverses.  Equation
\eqref{eq:binary-update} says simply that
\[
  \mA_g=\Phi_{\va_g,\va_g}.
\]
For example,
\[
  \mA_g\mA_h=\Phi_{\va_g\va_h,\va_h\va_g}.
\]
The order reversal in the right factor is the extra information stored by
the hidden state.

The pair \((L,R)\) determines \(\Phi_{L,R}\) up to the simultaneous sign
change \((L,R)\mapsto(-L,-R)\).  To see this, suppose
\(LqR=L'qR'\) for every \(q\).  With \(c=L^{-1}L'\), the case \(q=1\)
shows that the corresponding right-hand difference is \(c^{-1}\); the
general equality then says \(cq=qc\) for every quaternion.  Thus
\(c=\pm1\).  Denote the full finite group of such rotations by
\begin{equation}\label{eq:pair-group}
  \widehat\Gamma
  :=\frac{\widetilde A_5\times\widetilde A_5^{\mathrm{op}}}
          {\{(1,1),(-1,-1)\}},
\end{equation}
of order \(120^2/2=7200\).  Let \(\Gamma\) be the subgroup generated by the
sixty token matrices.  Then \(\Gamma\) is finite and every
\(\mQ\in\Gamma\) has the form \(\Phi_{L,R}\).

\paragraph{Step 5: decode only the left factor.}
Define
\begin{equation}\label{eq:left-decoder}
  p(\Phi_{L,R}):=[L]\in
  \widetilde A_5/\{\pm1\}\cong A_5.
\end{equation}
The simultaneous-sign ambiguity proves that \(p\) is well defined.
Equation~\eqref{eq:pair-composition} proves that it is a homomorphism, and
\begin{equation}
  p(\mA_g)=[\va_g]=g.
\end{equation}
Therefore, for every \(\mQ\in\Gamma\),
\begin{equation}\label{eq:matrix-tracking}
  p(\mA_g\mQ)=g\,p(\mQ).
\end{equation}
This is the desired state update: the decoder keeps the accumulated left
factor and discards the path-dependent right factor.

The decoder is genuinely many-to-one.  Choose noncommuting \(g,h\in A_5\)
and put \(k=(gh)^{-1}\).  The product
\(\mA_g\mA_h\mA_k\) has left factor
\(\va_g\va_h\va_k=\pm1\), so it decodes to the identity.  Its right factor
projects to
\begin{equation}
  khg=h^{-1}g^{-1}hg\neq e,
\end{equation}
so this hidden rotation is not the identity.  Thus the identity of \(A_5\)
already has at least two distinct hidden representatives.

\paragraph{Step 6: decode after the KDA query projection.}
Initialize the KDA matrix state at \(\mS_0=\mI\), set its additive writes to
zero, and use the transitions above.  After every word the state is some
\(\mQ\in\Gamma\).  Choose a fixed query \(\mathbf q\in\R^4\) with trivial
stabilizer under the full finite group \(\widehat\Gamma\).  Such queries
exist because the fixed spaces of the finitely many nonidentity matrices
cannot cover \(\R^4\).

The standard KDA output is
\[
  \mathbf o(\mQ)=\mQ^\top\mathbf q.
\]
This output uniquely determines \(\mQ\).  Indeed, if
\(\mQ_1^\top\mathbf q=\mQ_2^\top\mathbf q\), then
\(\mQ_2\mQ_1^\top\mathbf q=\mathbf q\).  Since
\(\mQ_2\mQ_1^\top\in\widehat\Gamma\) and the stabilizer of \(\mathbf q\) is
trivial, we obtain \(\mQ_1=\mQ_2\).

We may therefore define a decoder using only the query output:
\begin{equation}\label{eq:query-decoder}
  \pi(\mQ^\top\mathbf q):=p(\mQ).
\end{equation}
There is a convenient maxout expression for this decoder.  For each
\(g\in A_5\), form the 120-vector codebook
\[
  \mathcal C_g
  :=\{\mQ^\top\mathbf q:
       \mQ\in\widehat\Gamma,\ p(\mQ)=g\}.
\]
For an output \(\mathbf o\), define
\begin{equation}\label{eq:maxout-decoder}
  s_g(\mathbf o):=\max_{\mathbf c\in\mathcal C_g}
       \langle\mathbf c,\mathbf o\rangle,
  \qquad
  \pi_{\rm out}(\mathbf o):=\arg\max_{g\in A_5}s_g(\mathbf o).
\end{equation}
All codewords are unit vectors.  If
\(\mathbf o=\mQ^\top\mathbf q\) and \(p(\mQ)=g\), then \(s_g(\mathbf o)=1\),
while every other label has score strictly below one because the query orbit
is injective.  Thus \eqref{eq:maxout-decoder} is exactly
\eqref{eq:query-decoder} on every reachable output.  Computationally it is
one fixed linear map to $60\times120$ scores, max pooling over the 120 hidden
right-factor states, and a 60-way argmax.

The max pooling is necessary for this symmetric code.  Each
\(\mathcal C_g\) is centrally symmetric and therefore has mean zero.  A
strictly correct affine 60-way classifier would, after averaging its class
inequalities over \(\mathcal C_g\), require the bias of class (g) to exceed
every other bias.  Repeating this for every (g) is impossible.

Using \eqref{eq:matrix-tracking},
\[
  \pi((\mA_g\mQ)^\top\mathbf q)
  =p(\mA_g\mQ)
  =g\,p(\mQ)
  =g\,\pi(\mQ^\top\mathbf q),
\]
which is exactly \eqref{eq:tracking-quotient}.  The query projection therefore
loses no information needed by the decoder.  Finally, all transitions are
orthogonal and \(\Gamma\) is finite, so both the matrix-state and output
orbits are stable finite sets whose required precision does not grow with
sequence length.
\end{proof}

\subsection{Connection between Diagonal-Plus-Rank-One Matrices and signed KDA}\label{app:orthogonal-dplr}
\JS{Still need to go through it.}
Rank-one perturbations of orthogonal matrices have also appeared in
computer vision~\citep{schreiber2009robust}. We record the converse
characterization relevant to DPLR transitions.

\begin{proposition}[Orthogonal DPLR characterization]
\label{prop:orthogonal-dplr}
Let
\[
    \mA=\mD+\vu\vv^\top\in\mathbb{R}^{n\times n},
    \qquad
    \mD=\Diag(d_1,\ldots,d_n),
\]
and suppose $\mA^\top\mA=\mI$. Then there exist a unit vector
$\vk\in\mathbb{R}^n$ and a diagonal sign matrix
$\mS=\Diag(s_1,\ldots,s_n)$, $s_i\in\{-1,+1\}$, such that
\[
    \mA=(\mI-2\vk\vk^\top)\mS.
\]
Consequently, $\mA$ has at most one non-real conjugate pair of
eigenvalues.
\end{proposition}

\begin{proof}
If $\vu\vv^\top=0$, the claim is immediate. Otherwise let
$\mathcal I=\{i:v_i\neq0\}$. For $i\notin\mathcal I$, orthogonality
of the columns of $\mA$ gives $d_i\in\{-1,+1\}$ and $u_i=0$.
These coordinates therefore decouple, so assume $v_i\neq0$ for all
$i$.

For $n\le2$ the result follows directly from the classification of
$O(1)$ and $O(2)$; in particular, we write every
planar rotation as a Householder transformation times a coordinate
reflection. Assume henceforth $n\ge3$ and set $c=\norm{\vu}_2^2$.
Expanding $\mA^\top\mA=\mI$ gives
\[
    \mD^2-\mI+\mD\vu\vv^\top+\vv\vu^\top\mD
    +c\,\vv\vv^\top=0.
\]
For $i\neq j$, the $(i,j)$ entry implies
\[
    \frac{d_i u_i}{v_i}+\frac{d_j u_j}{v_j}=-c.
\]
Using three distinct indices shows that every term equals $-c/2$;
hence
\[
    \mD\vu=-\frac c2\vv.
\]
Substitution above gives $\mD^2=\mI$, so $\mS:=\mD$ is a diagonal
sign matrix. Taking norms in the preceding identity gives
$c\norm{\vv}_2^2=4$. Therefore, for
$\vk=\vv/\norm{\vv}_2$,
\[
    \mS\mA
    =\mI-\frac c2\vv\vv^\top
    =\mI-2\vk\vk^\top.
\]
Thus
\[
    \mA
    =\mS(\mI-2\vk\vk^\top)
    =\bigl(\mI-2(\mS\vk)(\mS\vk)^\top\bigr)\mS,
\]
which proves the claim after renaming $\mS\vk$.

Finally, if the $\pm1$ eigenspaces of $\mS$ have dimensions $p$ and
$n-p$, their intersections with $\vk^\perp$ have total dimension at
least $n-2$ and consist of real eigenvectors of $\mA$. Hence at most
two eigenvalues remain, giving at most one non-real conjugate pair.
\end{proof}

\begin{remark}
For example, \citet{schreiber2009robust} study rank-one perturbations
of rotations in computer vision. The proposition above instead
characterizes the intersection of the orthogonal group with the
diagonal-plus-rank-one family.
\end{remark}

\begin{theorem}[Persistent rotations in non-expansive DPLR]
\label{thm:dplr-persistent-pairs}
Let

$$
    \mA=\mD+\mR\in\mathbb{R}^{n\times n},
    \qquad
    \mD=\mD^\top \text{ diagonal},
    \qquad
    \operatorname{rank}(\mR)\le r,
$$

and suppose $\norm{\mA}\le1$. Then $\mA$ has at most $r$ non-real
conjugate pairs of eigenvalues on the unit circle. In particular, a
non-expansive rank-one DPLR transition has at most one such pair.
\end{theorem}

\begin{proof}
Let $\mathcal W$ be the real invariant subspace corresponding to the
unit-circle eigenvalues of $\mA$. If
$\mA\vx=\lambda\vx$ with $|\lambda|=1$, then
$\norm{\mA\vx}_2=\norm{\vx}*2$. Since
$\mA^\top\mA\preceq\mI$, equality implies
$\mA^\top\mA\vx=\vx$, and hence
$\mA^\top\vx=\bar{\lambda}\vx$. Thus $\mathcal W$ reduces $\mA$ and
$\mA|*{\mathcal W}$ is orthogonal.

Since $\mD$ is symmetric,

$$
    \mA-\mA^\top=\mR-\mR^\top,
    \qquad
    \operatorname{rank}(\mA-\mA^\top)\le2r.
$$

Therefore

$$
    \operatorname{rank}\!\left(
        \mA|_{\mathcal W}-(\mA|_{\mathcal W})^\top
    \right)\le2r.
$$

In a real orthonormal basis, $\mA|_{\mathcal W}$ is a direct sum of
$\pm1$ blocks and planar rotation blocks. Each nontrivial rotation
block contributes rank $2$ to the skew-symmetric part, while the
$\pm1$ blocks contribute zero. Hence, if $c$ is the number of
non-real conjugate pairs on the unit circle,

$$
    2c
    =
    \operatorname{rank}\!\left(
        \mA|_{\mathcal W}-(\mA|_{\mathcal W})^\top
    \right)
    \le2r,
$$

so $c\le r$.
\end{proof}

\begin{remark}
The theorem constrains persistent rather than total spectral
complexity. Additional non-real pairs may lie strictly inside the unit
disk and are therefore damped.
\end{remark}


\section{The Window for Complex Eigenvalues}\label{sec:setup}
Now, we want to find the eigenvalue decomposition of $\mA = (\mI- \beta \vk \vk^\top ) \Diag(\valpha)$ with $\beta \in \left[0, 2\right], \alpha_i \in \left[-1, 1\right]$ and $\lVert \vk \rVert =1$.
 We will show the following theorems:
 \begin{theorem}[Complex Eigenvalues in Diagonal Householder product]
 \label{thm:complex_eigenvalues}
 The eigenvalue decomposition of $\mA = (\mI- \beta \vk \vk^\top ) \Diag(\valpha)$ has at most one pair $\lambda, \lambda^{*}$ of complex eigenvalues with non-zero imaginary part, and only if both $\beta \in \left[1, 2\right]$ and any $\alpha_i < 0$.
 \end{theorem}\label{th:gate_plus_householder}
 This means it is not sufficient to extend $\beta \in \left[0, 2\right]$ alone within KDA as in \citet{grazzi2025}, nor is it sufficient to just extend the range of $\alpha_i$. This is similar to the requirement shown in~\citep[Prop 1.3]{siems2025}, showing that both $\beta$s in product of two generalized householders need to be greater than 1 for the product to obtain complex eigenvalues.

 \begin{proof}
 Note that $H^{\beta}_{\vk} := (\mI- \beta \vk \vk^\top )$ has eigenvalues $(1- \beta, 1,...)$, one eigenspace defined by $\vk$ (normalized) as eigenvector and the other subspace being the orthogonal subspace to this vector. So we can pick an orthogonal matrix $\mQ$, with $\vk$ as first column vector such that $\mQ H^{\beta}_{\vk} \mQ^\top = \Diag (1-\beta, 1, ...) $. So we can transform the eigenvector equation for $\mA$ as:
\begin{equation}
\label{eq:char_polynomial_eigenvalues}
\lambda \mQ \vx = \mQ \mH^{\beta}_{\vk} \overbrace{\mQ^\top \mQ}^{\mI} \Diag{\left(\valpha \right)} \vx = \Diag \left(1-\beta, 1, ...\right) \overbrace{\mQ  \Diag (\valpha) \mQ^\top}^{\mB} \mQ \vx
\end{equation}
We can apply a similarity transformation using the magnitudes of the generalized Householder $\mSigma := \Diag( |(1-\beta)|, 1, ..) $ , assuming $\beta \neq 1$, and substituting $\vy := \mSigma^{-\sfrac{1}{2}} \mQ \vx $:
\begin{equation}
\lambda \vy = \overbrace{\Diag( \sign (1 - \beta), 1, ...) }^{\mJ} \overbrace{\mSigma^{\sfrac{1}{2}} \mB (\mSigma^{\sfrac{1}{2}})^\top}^{\mS} \vy
\end{equation}

Since now $\mS$ is symmetric, its eigenvalues are real. Let's now take an eigenvector $\vx$ with eigenvalue $\lambda \notin \R, \lambda \in \C $ of $\mT := \mJ \mS$ that is complex. Then:
\begin{equation}
\vx^{*} \mJ \mT \vx = \lambda \vx^{*} \mJ \vx = \vx^{*} \overbrace{\mJ \mJ}^{\mI} \mS \vx \in \R
\end{equation}
This implies that $ \vx^{*} \mJ \vx = 0 $. For two eigenvectors of $\mT$ (and correspondingly $\mA$ through transformation with $\mQ$):
\begin{equation}
\mT \vx=\lambda \vx, \qquad \mT \vy=\mu \vy \implies (\mu - \overline{\lambda})\vx^{*} \mJ \vy = 0
\end{equation}
For $1 - \beta > 0$, this cannot be satisfied (for normalized eigenvectors) - so all eigenvalues have to be real. For the case $1 - \beta < 0$, the $\mJ$-neutral subspace is one-dimensional, so there can be at most one eigenvector with eigenvalue in the complex upper half plane, and one corresponding complex conjugated one in the lower half plane. 

Now to the opposite, if we keep $\forall i: \; \alpha_i > 0 $, it is also not possible to have complex eigenvalues. To see this, it this case we can apply another substitution for the eigenvalue equation, with $\mGamma = \Diag (\valpha ) > 0$ in $\vz = \mGamma^{-\sfrac{1}{2}} \vx$:

\begin{align}
 \lambda \vz = \overbrace{\mGamma^{\sfrac{1}{2}} \mH^{\beta}_{\vk} \mGamma^{\sfrac{1}{2}}}^{\mT} \vz
\end{align}

Since now $\mT$ is symmetric, so are its eigenvalues, meaning that also the eigenvalues of $\mA$ in this case are real.
\end{proof}





\section{One Layer Fewer: Automata Simulation}\label{app:wfamin}
\providecommand{\vc}{{\bm{c}}}

\paragraph{Lineage of the construction.}
The construction begins with a recurrent layer whose state determines the
current position $i\bmod 2m$. We call this the \emph{clock layer}; its output
tells the later layers which slot of a length-$2m$ block to read or update.
Together with a layer that buffers the recent tokens and a layer that
accumulates the selected matrix factors, it forms the
clock--buffer--accumulator construction shared by the three claims in
\Cref{thm:multilayer}. RWKV-7 introduced it for regular
languages \citep[Appendix~D]{peng2025rwkv7}. DeltaProduct adapted the same
block router to group word problems and, through a Krohn--Rhodes
decomposition, to arbitrary regular languages \citep[Thms.~1--2]{siems2025}.
Finally,
\citet[Thm.~6]{merrill_why_2026} extended it to arbitrary weighted finite
automata (WFAs) over $\mathbb Q$.

The common computation is matrix multiplication. Let $\mM_a$ be the
column-state transition of symbol $a$. Starting from
$\bm p_0=\bm\alpha_0$, the update
$\bm p_t=\mM_{w_t}\bm p_{t-1}$ matches the signed KDA recurrence in the main text,
and its readout is
\[
  \bm\omega^{\!\top}\bm p_t
  =\bm\omega^{\!\top}\mM_{w_t}\cdots\mM_{w_1}\bm\alpha_0
  .
\]
For a DFA, $\bm p_t$ is one-hot, the matrices describe deterministic maps, and
$\bm\omega$ selects the accepting states. For a finite group, the matrices are
permutations and the readout decodes their product. These are therefore three
instances of the same accumulator, not three unrelated constructions.

A DeltaNet step cannot apply a general $\mM_a$: its multiplicative transition
has the restricted form $\mI-\beta\vk\vk^{\!\top}$. The construction instead
buffers a block of $m$ symbols, computes its transition by a finite lookup,
factorizes that transition into at most $m$ permitted matrices, and streams one
factor per position during the next block. Note that the first steps of a sequence can always be handled through the feed forward-based lookup table, so it's sufficient to focus on transitions within full blocks in sequence. Two layers provide the position
modulo $2m$, a third stores the last $2m$ tokens and performs the lookup, and a
fourth accumulates the factors. A completion vector in the readout handles the
one-block delay. Here $m$ is the \emph{factor budget}: an upper bound on the
number of permitted recurrent matrices needed to factor any transition that a
block may produce. A shorter factorization is padded with identity steps so
that every block still has length $m$. Sufficient values for the different
matrix families are collected in
\Cref{thm:automata-factor-counts}.

Signed KDA changes only the clock. DeltaNet first computes parity and then uses
it to alternate two reflections. Signed KDA places one of those reflections in its
signed diagonal gate, so the following single layer advances directly through
the $2m$ clock states. The buffer, accumulator, and completion readout are
unchanged.

\begin{lemma}[One-step modular counter]\label{lem:wfamincount}
For every $m$ there is a \emph{one}-layer signed KDA head whose readout determines
$i\bmod 2m$ at every position $i$.
\end{lemma}
\begin{proof}
With $\beta=2$, $\valpha=(1,-1)$ and
$\vk=(-\sin\tfrac{\varphi}{2},\cos\tfrac{\varphi}{2})^{\!\top}$ the transition
$(\mI-2\vk\vk^{\!\top})\Diag(\valpha)$ is rotation by $\varphi$. Set
$\varphi=\pi/m$ and $\vc_0=\ve_1$. Then
$\vc_i=(\cos(\pi i/m),\sin(\pi i/m))^{\!\top}$ visits $2m$ distinct points.
Queries $\ve_1,\ve_2$ expose the coordinates, and a finite lookup returns the
residue.
\end{proof}

This is the one-layer counterpart of the $n_h\ge2$ DeltaProduct counter in
\citet[Lem.~2(ii)]{siems2025}. Merrill et al.'s DeltaNet router instead obtains
the same rotation from two alternating reflections, which requires the parity
layer beneath it \citep[Lem.~7]{merrill_why_2026}. For general $m$, these
rotation parameters are algebraic. Thus ``finite precision'' here uses the
exact finite-datatype convention of \citet[Appendix~A.4]{grazzi2025}; it is not
a robustness claim for an arbitrary floating-point implementation.

For the accumulator we use the DeltaProduct permutation factorization
\citep[Thm.~3]{siems2025}, the RWKV-7 identity--swap--copy decomposition
\citep[Lems.~3--4]{peng2025rwkv7}, and the rational DeltaNet program
\citep[Lems.~9--12 and Thm.~11]{merrill_why_2026}. In the unit-key convention, the
latter contains factors whose effective DeltaNet learning rate $\beta$
exceeds $2$
\citep[Lem.~10]{merrill_why_2026}.
This explains the $\beta>2$ condition
in the regular-language and WFA clauses of \Cref{thm:multilayer}; the group
construction uses only $\beta=2$ reflections.

We first record the factor budgets that determine $m$. RWKV-7 applies each
identity, swap, or copy primitive in one step \citep[Lem.~4]{peng2025rwkv7}.
Merrill et al. use $2n$ RWKV-7 overwrite factors for a general rational matrix
\citep[Lems.~5--6 and Thm.~9]{merrill_why_2026}; for DeltaNet they implement a
unit coordinate addition with three factors and a general rational $n\times n$
matrix with $8n^2+5n+1$ factors
\citep[Lems.~10--12]{merrill_why_2026}. A coordinate copy first clears its
destination and then applies three Householder factors. GDN must use a separate
transition for the clear. Signed KDA performs the clear and the first Householder in
the single transition $\mathcal H_2(\ve_s+\ve_d)
(\mI-\ve_d\ve_d^{\!\top})$, for source $s$ and destination $d$, reducing the
copy from four steps to three. The $3n$ exact-real GDN bound below is also the
norm-bounded matrix factorization in \citet[Prop.~1.2]{grazzi2025}.

\setcounter{theorem}{12}
\begin{theorem}[Factor budgets for the accumulator]\label{thm:automata-factor-counts}
Let $n$ be the automaton-state dimension. The following numbers of recurrent
matrix factors are sufficient:
\[
\begin{array}{lccc}
\toprule
\text{matrix family or primitive} & \text{RWKV-7} & \text{DeltaNet/GDN} & \text{signed KDA}\\
\midrule
\text{one transposition} & 1 & 1 & 1\\
\text{arbitrary permutation} & n-1 & n-1 & n-1\\
\text{one coordinate copy} & 1 & 4 & 3\\
\text{deterministic transition, explicit construction} & n & 4n & 3n\\
\text{deterministic transition, exact-real SVD} & n & 3n & 2n\\
\text{arbitrary rational }n\times n\text{ matrix} & 2n & 8n^2+5n+1 & 7n^2+3n\\
\bottomrule
\end{array}
\]
Over exact real arithmetic the SVD route lowers the deterministic-transition
budgets to $3n$ for GDN and $2n$ for signed KDA, but it does not by itself provide the
rational precision guarantee of the explicit construction. All entries are
upper bounds.
\end{theorem}
\begin{proof}
Write $\mathcal H_\gamma(\vu)=\mI-\gamma\vu\vu^{\!\top}$. A signed KDA factor is
$\mathcal H_\gamma(\vu)\mD$: it applies the diagonal first and the
Householder second.

\textit{Transpositions and permutations.}
A transposition is $\mathcal H_1(\ve_i-\ve_j)$, so a permutation costs at
most $n-1$ factors.

\textit{Coordinate copies.}
For $s\ne d$, let $\mC_{s\to d}$ denote the copy matrix that maps
$x_d\leftarrow x_s$ and leaves every other coordinate unchanged. Set
$\vu=\ve_s+\ve_d$, $\vw=\ve_s+2\ve_d$, and
$\mD_d=\mI-\ve_d\ve_d^{\!\top}$. The identity
\[
 \mI+\ve_d\ve_s^{\!\top}
 =\mathcal H_{1/3}(\vw)\mathcal H_{1/2}(\ve_s)\mathcal H_2(\vu)
\]
is the column-state transpose of the three-factor transvection in
\citet[Lem.~10]{merrill_why_2026} and gives
$\mC_{s\to d}=(\mI+\ve_d\ve_s^{\!\top})\mD_d$.
GDN uses $\mD_d=\mathcal H_1(\ve_d)$ as a fourth factor, whereas signed KDA
combines the clear and the first Householder into the single factor
$\mathcal H_2(\vu)\mD_d$. Thus a copy costs four GDN factors and three signed
KDA factors.

\textit{Deterministic transitions: explicit construction.}
The RWKV-7 decomposition uses at most $n$ identity, transposition, or copy
primitives \citep[Lems.~3--4]{peng2025rwkv7}. Applying the preceding copy
costs gives $4n$ factors for GDN and $3n$ for signed KDA.

\textit{Deterministic transitions: exact-real SVD.}
For the exact-real bounds, write $\mM=\mU\mSigma\mV^{\!\top}$ and multiply
$\mM$ by a positive constant so that the scaled singular values lie in
$[0,1]$; this common scale is immaterial to DFA recognition. The two
orthogonal factors cost at most $n$ reflections each. GDN uses another $n$
generalized Householders for the diagonal, whereas signed KDA absorbs that diagonal
into the adjacent reflection on its left, giving $3n$ and $2n$.

\textit{Arbitrary rational matrices.}
The RWKV-7 entry is the $2n$-overwrite decomposition of
\citet[Lem.~6]{merrill_why_2026}. For DeltaNet, start from the
$8n^2+5n+1$-factor program of \citet[Lems.~11--12]{merrill_why_2026}: each
scaled addition uses two three-factor transvections, one coordinate scaling,
and one clear. Signed KDA combines the clear with the first Householder of the next operation,
reducing the cost from eight to seven factors. The scaling remains separate:
its rational coefficient is arbitrary and need not lie in signed KDA's bounded
diagonal-gate range. Signed KDA's channel-wise diagonal also clears all scratch and
temporary coordinates at once initially. At the end, the last temporary clear
and all main-coordinate clears are combined with the first of the $3n$
copy-back factors. The total is therefore $7n^2+3n$.
\end{proof}

\setcounter{theorem}{11}
\begin{proposition}[Three layers suffice]\label{prop:wfamin}
A three-layer signed KDA stack with the extended gate and learning-rate ranges solves
every finite group-word problem under the exact finite-datatype convention above. If DeltaNet learning
rates $\beta>2$ are
allowed, it also recognizes every regular language in that convention and,
under rational-number arithmetic,
computes the value of every WFA over $\mathbb{Q}$ in polynomial precision.
\end{proposition}
\begin{proof}
Start from the four-layer DeltaNet WFA simulation of
\citet[Thm.~11]{merrill_why_2026}, including its rational-number and polynomial-precision
assumptions, and replace its two clock layers by \Cref{lem:wfamincount}. The remaining
layers stream, respectively, the permutation, DFA, or rational WFA factors
from \Cref{thm:automata-factor-counts}, using $m=n-1$, $m=3n$, and
$m=7n^2+3n$, respectively. Their completion readouts then decode the group
element, DFA state, or WFA value.
\end{proof}

This proves \Cref{thm:multilayer}. The matrix family changes only the final
accumulator, its completion readout, and the required value of $m$; the
one-layer signed KDA clock is shared by all three cases.

The clock layer cannot be removed from GDN. A unary WFA can already have a
periodic output, whereas a fixed GDN transition has only real eigenvalues. The
following proposition is the $L=1$, fixed-input specialization of
\citet[Thm.~2 and Appendix~B.2]{grazzi2025}: in their finite-precision model,
a one-layer state with real spectrum is eventually at most two-periodic.
\setcounter{theorem}{10}
\begin{proposition}[A real spectrum forces the second layer]\label{prop:wfaminreal}
Let a finite-precision layer have position-independent parameters and transition
$\mA$ with $\spec(\mA)\subset\R$ --- in particular Gated DeltaNet
\citep[Eq.~(10)]{yang2025gdn}, $\mA=\alpha(\mI-\beta\vk\vk^{\!\top})$,
\emph{including} the widened scalar range $\alpha\in[-1,1]$, and DeltaNet at
$\alpha=1$. On a fixed unary input, its state and every fixed decoder output
are eventually periodic with period dividing $2$. In particular, the layer
cannot count modulo $q$ for any $q>2$.
\end{proposition}
\begin{proof}
With a fixed write $\vb$,
\[
  \mH_i=\mA^i\mH_0+\sum_{j<i}\mA^j\vb .
\]
In Jordan form, every entry is a finite sum of terms $p(i)\lambda^i$, with
$p$ a polynomial and $\lambda\in\R$ (see also \Cref{thm:complex_eigenvalues}). After casting to a fixed finite datatype,
each such term is eventually constant on the even and odd subsequences: its
magnitude either vanishes, saturates, or stays constant, while its sign can
only alternate when $\lambda<0$. Hence $\mH_i$ eventually alternates between
at most two states, and so does any fixed decoder. A single GDN layer therefore
cannot supply the $2m$-state clock used in \Cref{prop:wfamin}.
\end{proof}

The scalar GDN gate commutes with the Householder factor, so widening either
scalar range preserves a real spectrum. GDN therefore needs the parity layer
to alternate two reflections. Signed KDA's channel-wise sign performs that
alternation within one transition; see also
\Cref{thm:complex_eigenvalues}.
\setcounter{theorem}{13}

\section{The Signed Gate Needs No Kernel Change}\label{app:gauge}
Previous work by~\citet{grazzi2025}, which signed the gate in Mamba~1 to demonstrate that this allows learning parity, pointed out that since the gates are usually kept in log-space for numerical accuracy for models like Mamba~2 and mLSTM, kernel changes are required to test the effectiveness of the signed gate. We show that the signed gate can be computed without any changes to the FlashKDA~\citep{flashkda2026} CUTLASS kernel interfaced through flash-linear-attention~\citep{yang2024fla}; however, a change of variables on the state is required. Write
$\Diag(\valpha_i)=\mS_i\mD_i$ with $\mS_i=\Diag(\vsigma_i)$, $\vsigma_i\in\{\pm1\}^{n}$ and
$\mD_i=\Diag(\abs{\valpha_i})$, and let $\mP_i=\mS_1\cdots\mS_i$ with $\mP_0=\mI$, so that
$\mP_i^{\!\top}=\mP_i=\mP_i^{-1}$.

\begin{lemma}[Sign gauge]\label{lem:gauge}
Let $\mH_i=(\mI-\beta_i\vk_i\vk_i^{\!\top})\mS_i\mD_i\mH_{i-1}+\beta_i\vk_i\vv_i^{\!\top}$ with
readout $\vo_i=\mH_i^{\!\top}\vq_i$, and put $\tilde\mH_i=\mP_i\mH_i$, $\tilde\vk_i=\mP_i\vk_i$ and
$\tilde\vq_i=\mP_i\vq_i$. Then
\[
\tilde\mH_i=\bigl(\mI-\beta_i\tilde\vk_i\tilde\vk_i^{\!\top}\bigr)\mD_i\tilde\mH_{i-1}
+\beta_i\tilde\vk_i\vv_i^{\!\top},
\qquad \vo_i=\tilde\mH_i^{\!\top}\tilde\vq_i ,
\]
with $\tilde\mH_0=\mH_0$, $\norm{\tilde\vk_i}=\norm{\vk_i}$ and $\mH_i=\mP_i\tilde\mH_i$.
\end{lemma}
\begin{proof}
Left-multiply the recurrence by $\mP_i$ and substitute $\mH_{i-1}=\mP_{i-1}\tilde\mH_{i-1}$.
Diagonal matrices commute, hence $\mS_i\mD_i\mP_{i-1}=\mD_i\mP_i$, and inserting $\mP_i\mP_i=\mI$
splits the transition as
$\bigl(\mP_i(\mI-\beta_i\vk_i\vk_i^{\!\top})\mP_i\bigr)\bigl(\mP_i\mD_i\mP_i\bigr)
=\bigl(\mI-\beta_i\tilde\vk_i\tilde\vk_i^{\!\top}\bigr)\mD_i$,
using $\mP_i\vk\vk^{\!\top}\mP_i=(\mP_i\vk)(\mP_i\vk)^{\!\top}$ and $\mP_i\mD_i\mP_i=\mD_i$. The
write term is $\beta_i\mP_i\vk_i\vv_i^{\!\top}$, and the readout is
$\vo_i=\mH_i^{\!\top}\vq_i=\tilde\mH_i^{\!\top}\mP_i\vq_i$. Orthogonality of $\mP_i$ gives the norm
identity, and $\mP_0=\mI$ the initial condition.
\end{proof}

\paragraph{Prior use.} Absorbing a cumulative gate into keys and queries is standard.
\citet{su2024rope} split a fixed-frequency rotation as
$\vq_t^{\!\top}\mR^{t-\tau}\vk_\tau=(\mR^{t}\vq_t)^{\!\top}(\mR^{\tau}\vk_\tau)$;
\citet{sun2023retentive} split a constant complex phase the same way, leaving the decay magnitude in
the mask; \citet[Prop.~3]{lahoti2026mamba} make the rotation data-dependent, showing that a complex
SSM equals a real scalar-transition SSM with rotary embeddings on $B$ and $C$; and
\citet{movahedi2025srope} split a learned input-dependent rotation across query and key and apply it
to Gated DeltaNet. Chunkwise kernels absorb the decay magnitude likewise, but only within a chunk,
the cumulative ratios being otherwise numerically unstable \citep{gla}. 
\Cref{lem:gauge} holds for any orthogonal $\mP_i$ commuting with the decay, so what is specific here
is the group. A rotation block commutes only with a decay constant on its plane, which the complex
parameterisations satisfy by construction at the price of half the rates, $n$ real dimensions
carrying $n/2$ decay magnitudes; signs commute with any channel-wise diagonal, so KDA's $n$ rates
survive intact. The reflection passes through by
$\mP_i(\mI-\beta_i\vk_i\vk_i^{\!\top})\mP_i^{\!\top}=\mI-\beta_i(\mP_i\vk_i)(\mP_i\vk_i)^{\!\top}$,
and $\mP_i$ costs no parameters, being the sign the decay gate already carries.

\paragraph{Computational Cost.} The kernel runs on $\abs{\valpha_i}$ and never sees a sign, so the costs lie outside it. $\mP_i$ is an integer parity prefix scan over the sign bits, retained by the backward pass at one byte per gate element, with two elementwise sign flips on $\vk_i$ and $\vq_i$ in each direction and an un-gauging of the cached state on exit. The key and query normalisation remain fused in the kernel, since $\ell_2$ norms are computed from squares and commute with $\mP_i$ exactly, and the bounded-gate TensorCore path, which the signed gate qualifies for and the shipped unbounded activation does not. No parameters, matrix multiplications or recurrent state are added. 

\section{The Key Activation influences the difficulty of learning group word problems}\label{app:silu}

The key path of DeltaNet~\citep{yang2024deltanet}, inherited by KDA, is $\vx\to\mW_k\to\mathrm{silu}\to\ell_2$. Since $\mathrm{silu}\ge-0.2785$, normalisation turns that floor into an angular prior: a unit key with a negative component of size $c$ requires $\norm{\mathrm{silu}(\vz)}\le0.2785/c$. Nothing is unreachable, since the map is onto the sphere, but the two groups fall on opposite sides. At $\beta=2$, $S_3$ needs no negative component at all: $\vk\in\{(\tfrac{\sqrt3}{2},0,\tfrac12),(\tfrac12,0,\tfrac{\sqrt3}{2}),\ve_3\}$ realises all five non-identity elements, the two of order $3$ reusing the first two keys. $S_4$ cannot avoid them because KDA requires mixed signed keys in order to represent it.

\citet{dubinin2026} report BD-LRU solving $S_4$ from $3$k samples versus DeltaProduct$_4$'s $0.130$, attributed to low-rank transitions being less sample-efficient than dense blocks. But DeltaProduct shares the same key path, while BD-LRU's entrywise gating has none to constrain. We instead attribute the gap to the bias silu imposes on the key direction.

\section{Experimental Details}\label{app:exp}

\begin{table}[h!]
\centering
\label{tab:model-configs}
\resizebox{\linewidth}{!}{%
\begin{tabular}{lccccc}
\toprule
\textbf{Config} & \textbf{Dense Attention} & \textbf{GDN} & \textbf{DeltaProduct} & \textbf{KDA} & \textbf{Signed-KDA} \\
\midrule
Hidden size                 & 768   & 768   & 768   & 768   & 768   \\
Num.\ hidden layers         & 28    & 28    & 28    & 28    & 28    \\
Num.\ attention heads       & 12    & 12    & 12    & 12    & 12    \\
Intermediate size           & 3072  & 2816  & 2816  & 3072  & 2816  \\
Hidden activation           & SwiGLU & SwiGLU & SwiGLU & SwiGLU & SwiGLU \\
RoPE $\theta$                & 10{,}000 & N/A & N/A & N/A & N/A \\
Max.\ position embeddings   & 2048  & 2048  & 2048  & 2048  & 2048  \\
Vocabulary size             & 50{,}304 & 50{,}304 & 50{,}304 & 50{,}304 & 50{,}304 \\
\midrule
Total parameters (millions)            & 341.55    & 342.33    & 342.07    & 344.87    & 344.87    \\
\bottomrule
\end{tabular}%
}
\caption{Configurations of each architecture used in our language modeling experiments are given above. The intermediate size, i.e., the latent dimension of the SwiGLU MLP block is reduced to match total parameter count for GDN and Signed-KDA models. To optimize the models, we use AdamW with a global batch size of 64, learning rate $5e-4$ following WSD: 2000 warmup steps and cooldown for the last $20\%$  of the token budget. Weight decay is set to $0.1$ and $(\beta_1, \beta_2)=(0.9, 0.95)$.}
\label{tab:arch_tab}
\end{table}

\begin{table}[h!]
\centering
\begin{tabular}{l|l}
\toprule
\textbf{Abbreviation} & \textbf{Full Name} \\
\midrule
Wiki. & WikiText \\
Lamb. & LAMBADA OpenAI \\
Hella. & HellaSwag \\
W.grad & WinoGrad \\
W.grande & WinoGrande \\
COPA & Choice of Plausible Alternatives \\
PIQA & Physical Interaction QA \\
ARC-e. & AI2 Reasoning Challenge (Easy) \\
ARC-c. & AI2 Reasoning Challenge (Challenge) \\
BBQA & BigBench QA \\
OBQA & OpenBook QA \\
Avg. & Average across accuracy tasks \\
\bottomrule
\end{tabular}
\caption{Full names of abbreviated evaluation benchmarks.}
\label{tab:lm_eval_names}
\end{table}



\pagebreak
\section{Additional Experimental Results}\label{appsec:exp_res}

\begin{table}[ht]
\centering
\caption{Length extrapolation on the group word problems. Scaled accuracy (chance $=0$, perfect $=1$) at sequence lengths $32$, $128$ and $512$; the training curriculum tops out at length $32$, so every column is extrapolation. Best of three seeds; one-layer models, $60$k steps, batch $1024$, Muon at learning rate $5\times10^{-3}$. Ranges in brackets are the eigenvalue ranges of the decay gate $\alpha$ and the Householder rate $\beta$. Best per column in bold.}
\label{tab:group_word_problems}
\resizebox{\linewidth}{!}{
\begin{tabular}{lccccccccc}
\toprule
 & \multicolumn{3}{c}{$S_3$} & \multicolumn{3}{c}{$S_4$} & \multicolumn{3}{c}{$A_5$} \\
\cmidrule(lr){2-4}\cmidrule(lr){5-7}\cmidrule(lr){8-10}
Transition & $32$ & $128$ & $512$ & $32$ & $128$ & $512$ & $32$ & $128$ & $512$ \\
\midrule
Gated DeltaNet\ \ $[-1,1]$ & 0.196 & 0.168 & 0.049 & 0.011 & 0.001 & 0.000 & 0.000 & 0.000 & 0.000 \\
DeltaProduct $n_h{=}2$\ \ $[-1,1]$ & \textbf{1.000} & \textbf{1.000} & \textbf{0.778} & 0.409 & 0.211 & 0.025 & \textbf{0.039} & 0.000 & 0.000 \\
\midrule
KDA \ \ $\alpha\in[0,1]$, \ \ $\beta\in[0,1]$ & 0.014 & 0.000 & 0.001 & 0.007 & 0.000 & 0.000 & 0.000 & 0.000 & 0.000 \\
KDA \ \ $\alpha\in[0,1]$, \ \ $\beta\in[0,2]$ & 1.000 & 0.288 & 0.154 & 0.068 & 0.037 & 0.000 & 0.000 & 0.000 & 0.000 \\
KDA \ \ $\alpha\in[-1,1]$, $\beta\in[0,1]$ & 0.999 & 0.754 & 0.211 & 0.181 & 0.004 & 0.000 & 0.000 & 0.000 & 0.000 \\
KDA \ \ $\alpha\in[-1,1]$, $\beta\in[0,2]$ & \textbf{1.000} & \textbf{1.000} & 0.772 & \textbf{1.000} & \textbf{0.985} & \textbf{0.297} & 0.001 & 0.000 & 0.000 \\
\bottomrule
\end{tabular}
}
\end{table}


\begin{figure}
    \centering
    \includegraphics[width=0.45\linewidth]{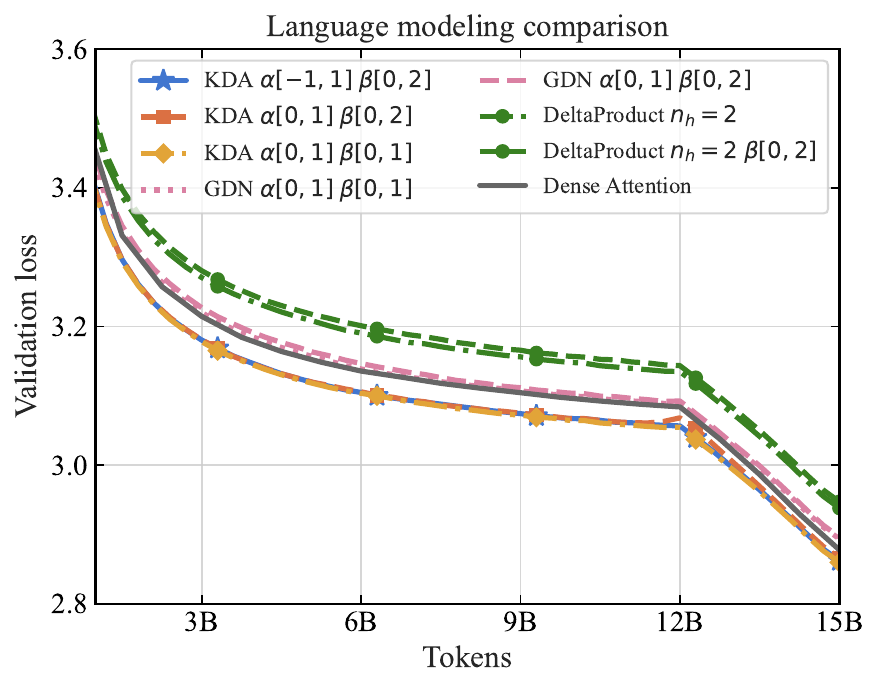}
    \includegraphics[width=0.45\linewidth]{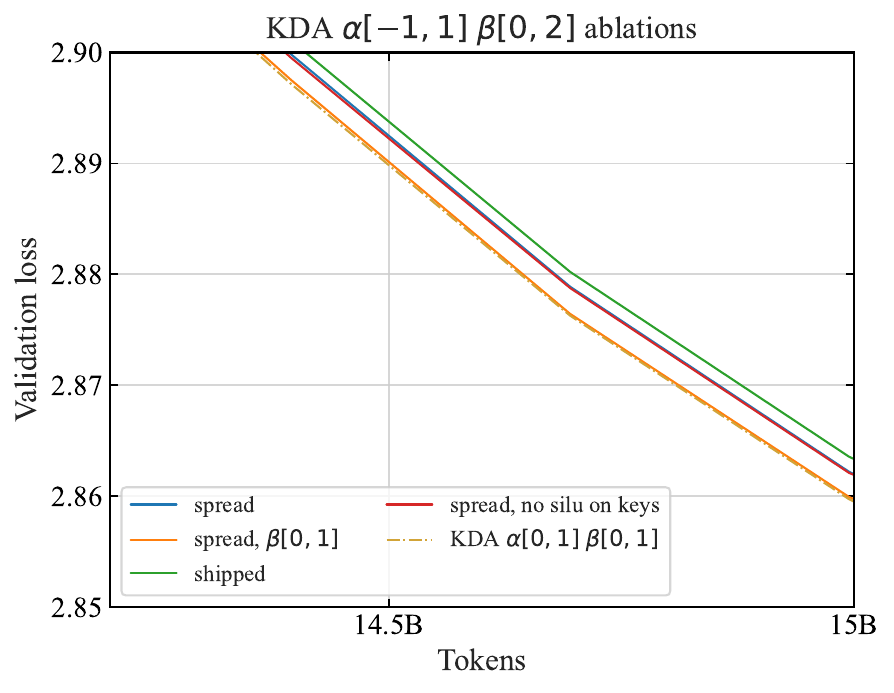}
    \caption{Language modeling results: validation loss versus tokens. (Left) Comparison across baselines. (Right) Comparison across ablations shown for the end of the cooldown phase, as loss values are quite close together.}
    \label{fig:val_curves}
\end{figure}

\section{Fused Kernels for the Signed Gate}\label{app:kernels}


\Cref{lem:gauge} keeps the sign out of the kernel but not out of the layer: $\mP_i$,
$\tilde\vk_i$ and $\tilde\vq_i$ are materialised before the call, two full-size tensors per layer in
each direction. \texttt{torch.compile} fuses the parity scan and both sign flips into the gate
epilogue and absorbs most of that; the kernels below remove the rest.

\paragraph{Placement.} The gauge goes into the $\ell_2$ normalisation rather than the recurrence.
That normalisation already writes the $\vq_i,\vk_i$ the chunk kernels read, and $\mP_i$ commutes
with it exactly, norms being computed from squares, so the flip costs one $\pm1$ read per element
and no new tensor. The chunkwise kernels, the WY representation and the state passing are unchanged,
and the parity leaves the state once at the chunk boundary. Outside the operator only the prefix
scan remains, resetting at sequence starts. In the backward $\mP_i$ is its own inverse and
$\langle d\tilde\vq_i,\tilde\vq_i\rangle$ is gauge-invariant, so a single leading factor is undone.

\begin{wrapfigure}[15]{r}{0.33\textwidth}
\centering
\vspace{-20pt}
\includegraphics[width=\linewidth, trim={3.5 3 0 0}, clip=true]{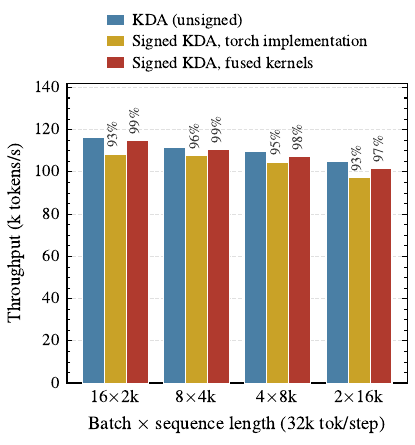}
\vspace{-20pt}
\caption{\small Training throughput of the $344$M signed-KDA model of \Cref{tab:arch_tab} at $32$k
tokens per step, one H200, \texttt{bfloat16}. Percentages are relative to unsigned KDA.}
\label{fig:kernel-throughput}
\end{wrapfigure}
\paragraph{Cost.} \Cref{fig:kernel-throughput} sweeps batch size against sequence length at fixed
tokens per step. The fused kernels hold $97$--$99\%$ of unsigned KDA's training throughput and
$93$--$98\%$ of its prefill, against $93$--$96\%$ and $89$--$94\%$ for the torch implementation.
All variants use \texttt{torch.compile}. The baseline uses the bounded gate so that all three take the same TensorCore path. 

\paragraph{Limits.} Computing the parity chunk-locally inside $\mathbf K\mathbf K^{\!\top}$ and the
output kernel drops the prefix scan but adds a sign read per consuming kernel, worth $0.3\%$ of a
step, and reaches into the output and state-passing kernels KDA shares with GLA and Gated DeltaNet.
The gauge is per value head, so grouped value attention needs $\vq_i,\vk_i$ expanded; the models
here have equal head counts.
