# Supplementary material for: Complex KDA: Understanding and Enhancing the Expressivity of Kimi Delta Attention
Source: arXiv:2609.24797 source file (2026-09-21)
Supplement: Supplementary file 5 [file appendix_wfa.tex]

\providecommand{\mC}{{\bm{C}}}\providecommand{\mF}{{\bm{F}}}
\providecommand{\mN}{{\bm{N}}}\providecommand{\mQ}{{\bm{Q}}}
\providecommand{\mV}{{\bm{V}}}\providecommand{\mX}{{\bm{X}}}
\providecommand{\mZ}{{\bm{Z}}}\providecommand{\vell}{{\bm{\ell}}}
\providecommand{\vc}{{\bm{c}}}\providecommand{\vd}{{\bm{d}}}
\providecommand{\vs}{{\bm{s}}}

\section{Automata in Three Layers}\label{app:wfa}

\Cref{thm:dichotomy} bounds what a \emph{single} step can be; a pipeline of $m$
steps is a different question. This section answers it constructively: the
signed gate recognises every regular, rational and stochastic language with
three layers, by spending $m$ tokens on one block of automaton transitions.
Throughout, $n$ is the number of automaton states and $d$ the head width, with
$d\ge n+1$ - the one place in this appendix where $n$ is not the head
dimension so that our proof is more in line with \citet{merrill_why_2026}, who are the first to proof a fixed number of GDN layers (with MLPs) can emulate a given WFA. Write $\mG_\beta(\vk)=\mI-\beta\vk\vk^{\!\top}$, so that the
transition of \Cref{sec:setup} is $\mA_i=\mG_{\beta_i}(\vk_i)\Diag(\valpha_i)$.

\paragraph{What is already known.} \citet{merrill_why_2026} place all linear RNNs
over $\mathbb{Q}$ in $\mathsf{PNC}^{1}$, show the DPLR family is
$\mathsf{PNC}^{1}$-complete, and give a $4$-layer DeltaNet
\citep{yang2024deltanet} simulating any weighted finite automaton, generalising
the regular-language construction of \citet{peng2025rwkv7}; the
permutation-diagonal family of \citet{terzic_structured_2025} is the deterministic corner of
the same picture. Their template - a modular counter, a cyclic buffer of
recent tokens, a finite lookup streaming one precomputed transition per token,
and an \emph{offline} factorisation of length-$m$ block products - is reused
verbatim below. What we don't use here is their arithmetic: their factors have
unnormalised keys and unbounded rate (the transvection gadget
$\mI-2\vu\vu^{\!\top}$ at $\vu=\ve_j+\ve_l$ has $\beta_{\mathrm{eff}}=4$ and
$\norm{\cdot}_2=3$), so they leave the box of \Cref{sec:setup} entirely. The
content of this section is that the same template runs \emph{inside} it, where
\Cref{lem:box} makes every step non-expansive and an expansive automaton
transition is therefore reachable only up to a positive scale. A clock
coordinate carries that scale, and the signed gate pays for itself twice: it
supplies a full signed diagonal per step and collapses their two counter layers
into one.

\paragraph{Assumptions.} As in \citet{merrill_why_2026}: the endpoints $0,\pm1,2$
and the finitely many constants in the factor tables are exact, arithmetic is
exact over $\R$, a wide enough feed-forward sublayer realises any map on a
finite input set, heads may be duplicated and coordinates padded, and a
beginning-of-sequence step initialises the states. A head starting at zero is
set to $\vh_0$ by one write, $\beta=1$, $\vk=\vh_0/\norm{\vh_0}$,
$\vv=\norm{\vh_0}$. The classifier reads the last data token; the construction
in fact scores every nonempty prefix.

\begin{lemma}[Primitives]\label{lem:wfaprim}
The gate of \Cref{sec:setup} realises exactly, in one step:
\textup{(P1)} any signed diagonal contraction $\Diag(\va)$, $\va\in[-1,1]^{d}$,
at $\beta=0$;
\textup{(P2)} any reflection $\mI-2\vk\vk^{\!\top}$, at $\beta=2$,
$\valpha=\mathbf 1$;
\textup{(P3)} the identity;
\textup{(P4)} a row overwrite
$\mH^{+}=(\mI-\ve_j\ve_j^{\!\top})\mH+\ve_j\vv^{\!\top}$, at $\beta=1$,
$\vk=\ve_j$, $\valpha=\mathbf 1$;
\textup{(P5)} the planar rotation by $\varphi$, at $\beta=2$,
$\valpha=(1,-1)$, $\vk=(-\sin\tfrac\varphi2,\cos\tfrac\varphi2)^{\!\top}$.
\end{lemma}
\begin{proof}
(P1)--(P4) are immediate; in (P1) the write term carries the factor $\beta$, so
any unit $\vk$ serves. (P5) is \Cref{lem:flip} at $q=1$, $n=2$, whose angle
$2\arccos\rho$ is $\varphi$ for $\rho=\cos(\varphi/2)$.
\end{proof}

(P1) and (P5) are what a pure Householder architecture lacks: coordinate scaling
costs one step per coordinate there \citep[Lem.~9]{merrill_why_2026} where (P1)
scales all $d$ at once, and the counter needs a parity layer beneath a layer of
alternating reflections \citep[Lem.~7]{merrill_why_2026} where (P5) rotates directly.

\paragraph{The controller.} Fix $m$. \emph{Layer~1} iterates (P5) at
$\varphi=\pi/m$ from $\vc_0=\ve_1$, so
$\vc_i=(\cos\frac{\pi i}{m},\sin\frac{\pi i}{m})^{\!\top}$ takes $2m$ distinct
values; two heads with queries $\ve_1,\ve_2$ expose them and a finite lookup
decodes $i\bmod 2m$. Its sign pattern is static, so it realises exactly a
$C_{2m}$ - the ceiling of \Cref{thm:static}, and all that is wanted - and by
\Cref{app:gauge} its parity degenerates to $(-1)^{i}$, leaving the kernel
untouched. \emph{Layer~2} keeps $\mZ_i\in\R^{2m\times d_v}$ and overwrites row
$1+((i-1)\bmod 2m)$ with $\phi(w_i)$ by (P4), $\phi$ an injective token code;
$2m$ duplicate heads with queries $\ve_j$ expose all rows, and with $i\bmod 2m$
a finite lookup recovers the last $2m$ symbols in order. \emph{Layer~3} is the
accumulator below.

\begin{definition}[Clock-compatible factorisation]\label{def:wfaclock}
Let $\vx_i=\mM_{w_i}\vx_{i-1}$ on $\R^{n}$, and for $u\in\Sigma^{m}$ put
$\mB_u=\mM_{u_m}\cdots\mM_{u_1}$ and
$\overline\mB_u=(\gamma_u\mB_u)\oplus[\gamma_u]$. The family is
clock-compatible if for each $u$ there are permitted transitions
$\mF_{u,j}=\mN_{u,j}\oplus[\gamma_{u,j}]$ on $\R^{n+1}$ with
$\gamma_{u,j}>0$ and a $\gamma_u>0$ such that
\begin{equation}
\mF_{u,m}\cdots\mF_{u,1}=\overline\mB_u .
\label{eq:wfaclock}
\end{equation}
The last coordinate is the clock.
\end{definition}

\begin{proposition}[Delayed block simulation]\label{prop:wfapipe}
Given clock-compatible length-$m$ factorisations, $\vell\in\R^{n}$ and
$\tau>0$, three signed-gate layers produce at every nonempty prefix a scalar
$y_i$ with
$\operatorname{sign}(y_i)=\operatorname{sign}(\vell^{\!\top}\vx_i-\tau)$.
\end{proposition}
\begin{proof}
Initialise $\vh_0=[\vx_0;1]$ and write $i=bm+r$ with $1\le r\le m$. During block
$b+1$ the accumulator applies $\mF_{u_b,1},\dots,\mF_{u_b,m}$, one per token,
where $u_b$ is the \emph{previous} complete block (identities while $b=0$), so
by \eqref{eq:wfaclock}
\[
\vh_i=\mF_{u_b,r}\cdots\mF_{u_b,1}\,
\overline\mB_{u_{b-1}}\cdots\overline\mB_{u_1}\vh_0 .
\]
The buffer holds $u_b$ together with the current partial block
$u'=w_{bm+1}\cdots w_i$ - at most $2m$ symbols, which is why the buffer has
that length - and Layer~1 supplies $r$, so the lookup returns both the next
factor and the correction
$\mC_i=(\mB_{u'}\oplus[1])\,\mF_{u_b,m}\cdots\mF_{u_b,r+1}$, which completes the
pending block and advances the partial one:
$\mC_i\vh_i=g_b\,[\vx_i;1]$ with $g_b=\prod_{j\le b}\gamma_{u_j}>0$. Put
$\va=[\vell;-\tau]$. Every factor is block diagonal, so the clock entry of
$\mC_i^{\!\top}\va$ is a negative multiple of $\tau$; hence
$\vq_i=\mC_i^{\!\top}\va/\norm{\mC_i^{\!\top}\va}$ is a legal unit query, is a
function of the lookup key, and
\begin{equation}
y_i=\vq_i^{\!\top}\vh_i
=\frac{g_b\bigl(\vell^{\!\top}\vx_i-\tau\bigr)}{\norm{\mC_i^{\!\top}\va}} .
\label{eq:wfascore}
\end{equation}
Both scales are positive.
\end{proof}

Unnormalised, $\mC_i^{\!\top}\va$ is the completion vector of \citet[\S C.4.4]{merrill_why_2026} and returns the automaton value itself; KDA forces
$\norm{\vq_i}=1$, so \eqref{eq:wfascore} is that value only up to the positive
factor $g_b/\norm{\mC_i^{\!\top}\va}$. Neither half of it is lost. Let
$c_i=(\mC_i)_{n+1,n+1}=\prod_{j>r}\gamma_{u_b,j}>0$ be the clock entry of the
correction; the last coordinate of $\mC_i\vh_i=g_b[\vx_i;1]$ says
$h_{i,n+1}=g_b/c_i$, which a duplicate head reads with the \emph{constant} unit
query $\ve_{n+1}$, this is what the clock is for. Dividing by it cancels the
unknown $g_b$, and both $c_i$ and $\norm{\mC_i^{\!\top}\va}$ are read off the
$\mC_i$ the lookup already computes:
\begin{equation}
\frac{y_i}{h_{i,n+1}}\cdot\frac{\norm{\mC_i^{\!\top}\va}}{c_i}
=\vell^{\!\top}\vx_i-\tau .
\label{eq:wfavalue}
\end{equation}
The value therefore costs one division, which the architecture has
anyway for normalisation \citep{merrill2026}, and only the \emph{sign} is
division-free. What does not transfer is the field: the reflections, their unit
normals and the scale $\gamma_u$ carry square roots, so \eqref{eq:wfavalue} is
real-algebraic arithmetic even for a rational automaton, where
\citet{merrill_why_2026} stay in $\mathbb{Q}$ at polynomial precision.

\begin{lemma}[Factorisation inside the box]\label{lem:wfafactor}
\textup{(F1)} If $\mB\in\{0,1\}^{n\times n}$ has exactly one $1$ per column then
$n^{-1/2}\mB$ is a product of $n-1$ reflections followed by one signed diagonal
contraction. \textup{(F2)} Any $\mX$ with $\norm{\mX}_2\le1$ is a product of at
most $2n-2$ reflections and one signed diagonal contraction.
\end{lemma}
\begin{proof}
(F1) Distinct rows of $\mB$ have disjoint supports, so with $d_j=\norm{\vb_j}$
the nonzero rows $\vb_j/d_j$ are orthonormal; completing them gives
$\mB=\Diag(\vd)\mQ$ with $\mQ\in O(n)$ and
$d_j=\sqrt{\#\{1\text{'s in row }j\}}\le\sqrt n$. Householder QR
\citep{householder1958} of $\mQ^{\!\top}$ has a diagonal sign matrix for its
triangular factor, and reflections are symmetric and self-inverse, so
$\mQ=\Diag(\vsigma)\mG_{n-1}\cdots\mG_1$ - the constructive
Cartan--Dieudonn\'e theorem, with the $n$-th reflection absorbed into the sign
diagonal, which (P1) supplies free. Then
$\mD_\star=n^{-1/2}\Diag(\vd\odot\vsigma)$ has entries in $[-1,1]$ and
$\mD_\star\mG_{n-1}\cdots\mG_1=n^{-1/2}\mB$. (F2) The same QR applied to both
factors of an SVD $\mX=\mU\Diag(\vs)\mV^{\!\top}$ gives
$\mX=\mG_1\cdots\mG_{n-1}\mD_\star\mG'_{n-1}\cdots\mG'_1$ with
$\mD_\star=\Diag(\vsigma_1\odot\vs\odot\vsigma_2)$, whose entries are signed
singular values. Schedule right to left, padding with identities.
\end{proof}

\begin{corollary}[Clock augmentation: the factors $\mF_{u,j}$]\label{cor:wfaclock}
Let $\gamma\in(0,1]$ and let $\gamma\mB=\mD_\star\mG_{n-1}\cdots\mG_1$ by
\textup{(F1)}, or $\gamma\mB=\mG_1\cdots\mG_{n-1}\mD_\star\mG'_{n-1}\cdots\mG'_1$
by \textup{(F2)}. Reading that product right to left and padding every
reflection as $\mG\oplus[1]$ and the single diagonal as
$\mD_\star\oplus[\gamma]$ defines factors $\mF_{u,1},\dots,\mF_{u,m}$ that are
clock-compatible in the sense of \Cref{def:wfaclock}: $m=n$ at
$\gamma=n^{-1/2}$ for column-one-hot $\mB$, and $m=2n-1$ at
$\gamma=1/\max\{1,\norm{\mB}_2\}$ in general.
\end{corollary}
\begin{proof}
$\mG\oplus[1]=\mI-2\tilde\vk\tilde\vk^{\!\top}$ for $\tilde\vk=[\vk;0]$, again a
unit normal, so (P2) permits it; $\mD_\star\oplus[\gamma]$ has all entries in
$[-1,1]$ because those of $\mD_\star$ do and $\gamma\le1$, so (P1) permits it.
Both are block diagonal with positive clock entries $1$ and $\gamma$, giving
\eqref{eq:wfaclock} with $\gamma_{u,j}\in\{1,\gamma\}$. No factor but the
diagonal touches the clock, so the product's clock entry is $\gamma$ and its
upper block is the product of \Cref{lem:wfafactor}, namely $\gamma\mB$; that is
$\overline\mB_u$.
\end{proof}

Deterministic transitions are expansive - $\mB=\bigl(\begin{smallmatrix}1&1\\
0&0\end{smallmatrix}\bigr)$ has $\norm{\mB}_2=\sqrt2$ - and (F1) is exactly
normalised mixing followed by erasure,
$2^{-1/2}\mB=\Diag(1,0)\cdot2^{-1/2}\bigl(\begin{smallmatrix}1&1\\
1&-1\end{smallmatrix}\bigr)$, where the unscaled copy available off the box is
not.

\begin{theorem}[Three-layer recognition]\label{thm:wfa}
Under the assumptions above, a three-layer signed-gate stack recognises
\textup{(a)} every language of an $n$-state DFA, with block length $m=n$ and
constant scale $\gamma_u=n^{-1/2}$; \textup{(b)} every language of an $n$-state
NFA, with $m=2n-1$ and $\gamma_u=1/\max\{1,\norm{\mB_u}_2\}$, without the subset
construction; and \textup{(c)} every strict-cutpoint language of an $n$-state
PFA \citep{rabin_probabilistic_1963}, with the same $m$.
\end{theorem}
\begin{proof}
(a) A product of column-one-hot matrices is column-one-hot, so (F1) and
\Cref{cor:wfaclock} apply to every $\mB_u$ at $m=n$, $\gamma_u=n^{-1/2}$. The
state
$\vx_i=\mM_{w_i}\cdots\mM_{w_1}\vx_0$ is one-hot, so \Cref{prop:wfapipe} at
$\vell=2\vf$, $\tau=1$ returns the sign of $2\vf^{\!\top}\vx_i-1=\pm1$ for the
accepting indicator $\vf$, which is the DFA decision. (b) Take
$\mM_\sigma[j,l]=1$ iff $l\xrightarrow{\sigma}j$, so
$\vf^{\!\top}\vx_i\in\mathbb{N}$ counts accepting runs - linear, where the
Boolean update $\mathbf 1[\mM_\sigma\vb>0]$ is not. Now (F2) and
\Cref{cor:wfaclock} apply at $m=2n-1$; at $\vell=2\vf$, $\tau=1$ the score is
positive iff some accepting run exists. (c) For a column-stochastic $\mM_\sigma$,
same factorisation, $\vell=\vf$ and $\tau=\eta\in(0,1)$ the cutpoint.
\end{proof}

At a block boundary the accumulator is $g\,[\vp;1]$ with $g>0$: the distribution
is represented projectively, $\vp=\vh_{1:n}/h_{n+1}$, and a cutpoint test needs
no division because the clock carries the same scale. Between boundaries the
reflections make the coordinates signed - this is an algebraic simulation, not
a claim that every substep is stochastic.

\paragraph{What it costs.} Key dimensions $2$, $2m$ and $n+1$ for the three
layers, $d_v\ge\abs{\Sigma}$ for a one-hot token code, and $2m$ duplicate heads
for the buffer readout. The lookup is finite but wide: its key space has size
$(\abs{\Sigma}+1)^{2m}$, so the table is exponential in $n$ - a constant-depth
expressivity construction, not a parameter count. The block scale
$g_b=\prod_{j\le b}\gamma_{u_j}$ decays geometrically, so the sign of
\eqref{eq:wfascore} is exact over $\R$ but the margin underflows in finite
precision; a robust version needs an isolated-margin hypothesis, and for
cutpoints the margin can be arbitrarily small before any rescaling
\citep{rabin_probabilistic_1963}. The accumulator's signs are data-dependent, so it needs the
gauge of \Cref{lem:gauge}; Layers~1 and~2 do not.

\paragraph{Relation to the DeltaNet program.} \Cref{tab:wfa} makes the trade
explicit. Their $\Theta(n^{2})$ budget is the cost of building every scaled add
from unit transvections and single-coordinate scalings; (P1) collapses the
scalings into one step and (F1)--(F2) do the mixing with reflections, which is
the whole of the $\Theta(n^{2})\to\Theta(n)$ gap. It is bought with the clock
coordinate, one division for the value, and the move from $\mathbb{Q}$ to
real-algebraic constants.

\begin{table}[h]
\centering\small
\setlength{\tabcolsep}{4pt}
\begin{tabular}{@{}lll@{}}
\toprule
& \textbf{DeltaNet} \citep{merrill_why_2026} & \textbf{signed gate} (this work)\\
\midrule
factors & $\beta$ free, $\vk$ unnormalised
        & $\beta\in[0,2]$, $\norm{\vk}=1$, $\valpha\in[-1,1]^{d}$\\
step norm & unbounded (up to $3$) & $\le1$ \\
scalings per step & $1$ & $d$, by (P1)\\
steps per block & $8n^{2}+5n+1$ & $n$ (DFA), $2n-1$ (general)\\
counter & $2$ layers & $1$ layer, by (P5)\\
layers & $4$ & $3$\\
rescaling & none & clock coordinate\\
output & exact value, no division & sign free, value by \eqref{eq:wfavalue}\\
field & $\mathbb{Q}$, needs $\tfrac12,\tfrac13$ & real-algebraic\\
\bottomrule
\end{tabular}
\caption{The template of \citet[\S C.4]{merrill_why_2026} run inside the box of
\Cref{sec:setup}. The last row of \Cref{tab:variants} is the constraint; the
last three rows here are what it costs.}
\label{tab:wfa}
\end{table}

\begin{remark} [What this does and does not say about the gate]\label{rem:wfascope}
The construction needs $\beta=2$ throughout, i.e.\ the widened rate of
\citet{grazzi2025,upstage2026}; the \emph{signed decay} then saves one counter
layer and up to half the block length, since with $\valpha\ge0$ the sign matrix
$\Diag(\vsigma)$ of \Cref{lem:wfafactor} must be spent as up to $n$ further
reflections. So this is a constant-factor and depth statement, not a separation
of language classes: \Cref{thm:wfa} is subsumed by
\citet[Thm.~6]{merrill_why_2026} once the box is dropped. Clause~(a) is not even the
cheapest route to a DFA - PD-SSM \citep{terzic_structured_2025} realises every
column-one-hot transition in \emph{one} step where (F1) spends $n$, buying that
the way \citet{merrill_why_2026} do, by leaving the box, since $\norm{\mP\mD}_2$
reaches $\sqrt n$ with the merge matrix above as the smallest case. What the
pipeline adds is (b) and (c), the latter recognising languages that need not be
regular \citep{rabin_probabilistic_1963}, while multi-layer PD is confined to
$\mathsf{NC}^{1}$ \citep[Thm.~7]{merrill_why_2026}; whether that is a genuine
separation is the conditional $\mathsf{NC}^{1}$ versus $\mathsf{PNC}^{1}$
question. Nor does it contradict
\Cref{thm:dichotomy}: the block product $\mB_u$ is realised over $m$ tokens, not
in one step, which is why the $\mathsf{NC}^{1}$-hard word problem of
\citet{barrington1989} is reachable here while $A_5$ is not reachable in one
step (\Cref{prop:a5}). That same gap - one step versus a $\Theta(m)$-token
pipeline - is what makes DPLR recurrences $\mathsf{PNC}^{1}$-complete in
\citet{merrill_why_2026}. Spreading Householder factors over time rather than within
a step is also what separates this from DeltaProduct \citep{siems2025}: the same
factors, paid in latency instead of heads.
\end{remark}
