# Supplementary material for: Complex KDA: Understanding and Enhancing the Expressivity of Kimi Delta Attention
Source: arXiv:2609.24797 source file (2026-09-21)
Supplement: Supplementary file 6 [file appendix_wfa_red.tex]

\section{One Layer Fewer: Automata Simulation}\label{app:wfamin}
\providecommand{\vc}{{\bm{c}}}

\citet[Thm.~6]{merrill_why_2026} show that a $4$-layer DeltaNet
\citep{yang2024deltanet} or RWKV-7 \citep{peng2025rwkv7} computes the value
$f(w)$ of any $n$-state weighted finite automaton over $\mathbb{Q}$, by a
router-plus-arithmetic template: Layer~1 emits the parity of the position,
Layer~2 the residue $i\bmod 2m$, Layer~3 keeps a $2m$-slot cyclic token buffer
feeding a finite lookup, and Layer~4 applies one precomputed multiplicative
step per token, executing an offline factorisation of each length-$m$ block of
automaton transitions. We take that construction as given and change exactly
one thing: under the channel-wise signed gate of \Cref{sec:setup}, Layers~1
and~2 are a single layer.

\begin{lemma}[One-step modular counter]\label{lem:wfamincount}
For every $m$ there is a \emph{one}-layer KDA head whose readout determines
$i\bmod 2m$ at every position $i$.
\end{lemma}
\begin{proof}
With $\beta=2$, $\valpha=(1,-1)$ and
$\vk=(-\sin\tfrac{\varphi}{2},\cos\tfrac{\varphi}{2})^{\!\top}$ the transition
$(\mI-2\vk\vk^{\!\top})\Diag(\valpha)$ is the planar rotation by $\varphi$:
this is \Cref{lem:flip} at $q=1$ in $n=2$, where $\rho=\cos(\varphi/2)$ and the
rotation angle is $2\arccos\rho$. Take $\varphi=\pi/m$ and $\vc_0=\ve_1$, so
that $\vc_i=(\cos\frac{\pi i}{m},\sin\frac{\pi i}{m})^{\!\top}$ runs through
$2m$ distinct points. Two duplicate heads with queries $\ve_1,\ve_2$ expose the
two coordinates, and a finite lookup maps the $2m$ values to the residue.
\end{proof}

\begin{proposition}[Three layers suffice]\label{prop:wfamin}
Under the hypotheses of \citet[Thm.~11]{merrill_why_2026}, a $3$-layer KDA stack
computes $f(w)$ at every position.
\end{proposition}
\begin{proof}
A DeltaNet transition is the KDA transition of \Cref{sec:setup} at
$\valpha_i=\mathbf 1$, so Layers~3 and~4 of their construction,  the buffer
with its lookup, and the arithmetic layer with its offline block factorisation, are KDA layers verbatim, with the same parameters and the same correctness
argument. Their Layers~1 and~2 exist only to deliver $i\bmod 2m$ to the Layer~3
lookup, which \Cref{lem:wfamincount} does in one layer.
\end{proof}

The saving is not bookkeeping: it is the one place in the template where the architectures genuinely differ.
As arbitrary WFAs also include ones that have to recognize repetitions of the same input, this serves as counterexample for where a single layer for modular counting fails.
\begin{proposition}[A real spectrum forces the second layer]\label{prop:wfaminreal}
Let a layer have position-independent parameters and transition $\mA$ with
$\spec(\mA)\subset\R$ and $\mA$ diagonalisable --- in particular Gated DeltaNet
\citep{yang2025gdn}, $\mA=\alpha(\mI-\beta\vk\vk^{\!\top})$, by \Cref{cor:gdn},
\emph{including} the widened scalar range $\alpha\in[-1,1]$, and DeltaNet at
$\alpha=1$. Then no readout of that layer is
periodic in $i$ with minimal period greater than $2$; in particular it does not
compute $i\bmod 2m$ for $2m\ge3$.
\end{proposition}
\begin{proof}
With a fixed write $\vb$ the state is
$\mH_i=\mA^{i}\mH_0+\sum_{j<i}\mA^{j}\vb$, so in an eigenbasis every coordinate
is $a_\lambda+b_\lambda\lambda^{i}$ for real $\lambda$, with $a_\lambda+b_\lambda i$
in place of it when $\lambda=1$. Any linear readout is a real combination of
these, and such a function has minimal period $p$ only if $\lambda^{p}=1$ for
each $\lambda$ carrying a non-constant term, i.e.\ $\lambda\in\{\pm1\}$ and
$p\le2$.
\end{proof}

So Gated DeltaNet inherits the parity layer of \citet[Lem.~7]{merrill_why_2026} for
the same reason it inherits \Cref{cor:gdn}: a scalar gate commutes with every
$\vk\vk^{\!\top}$, the transition stays symmetric, and a real spectrum offers
only the frequencies $0$ and $\frac{1}{2}$. Widening the rate does not help. By
\Cref{lem:det} a finite-order step needs $\beta\in\{0,2\}$ and $\abs{\alpha}=1$,
which in the counter's plane leaves exactly $\pm\mI$ and
$\pm(\mI-2\vk\vk^{\!\top})$: two reflections, and one central rotation of angle
$\pi$. The obstruction is centrality rather than sign range --- $\Diag(\vsigma)$
turns a reflection into a rotation only when $\vsigma$ is \emph{non-constant},
and a scalar gate offers only $\vsigma=\pm\mathbf 1$. Equivalently, in
\Cref{lem:flip} the angle $\varphi=2\arccos\rho$ is set by the key's mass on the
flipped channels, and flipping all of them or none leaves $\rho\in\{0,1\}$.

Two reflections do of course compose to a rotation, which is exactly what
\citet[Lem.~7]{merrill_why_2026} exploit; but composing them requires alternating
$\vk$ with the position, so the alternating layer must be told $i\bmod 2$ by the
layer beneath it. That is the whole content of their first layer, and the whole
of the saving here: a channel-wise gate carries its own flip, so the reflection
and the sign meet inside a single step instead of across two. The depth of the
construction is therefore a direct reading of \Cref{tab:variants} --- the last
row buys a layer that no row above it can buy, and by \Cref{prop:main} it buys
it from the key geometry, the gate contributing only the signs.

\begin{remark}[Scope]\label{rem:wfaminscope}
Two caveats. First, \Cref{prop:wfamin} inherits the gate ranges under which
\citet{merrill_why_2026} state their Layer~4, namely unnormalised keys and
unrestricted $\beta$; that arithmetic is not non-expansive, and running the same
template inside the box of \Cref{sec:setup} additionally costs a clock
coordinate and $\Theta(n)$ steps per block, which is developed separately.
Second, \Cref{lem:wfamincount} uses a \emph{static} sign pattern, so by
\Cref{thm:static} it realizes exactly a $C_{2m}$ --- all a counter needs --- and
by \Cref{app:gauge} its parity prefix degenerates to $(-1)^{i}$, leaving the
shipped kernel untouched. The one-layer counter is thus free in every sense
except the sign range itself.
\end{remark}
